# Supplementary material for: Multiwavelength Study of Blue Straggler Stars in Tombaugh 2: Evidence for Binary Mass Transfer and Constraints on Cluster Dynamical State
Source: arXiv:2604.12494 source file (2026-04-14)
Supplement: Supplementary file 1 [file Appendix_A.tex]

\section{Single-Component SED Fits of Blue Straggler Stars}
\label{Appendix_SED}

\begin{figure*}[t]
    \centering
    \includegraphics[width=0.92\linewidth]{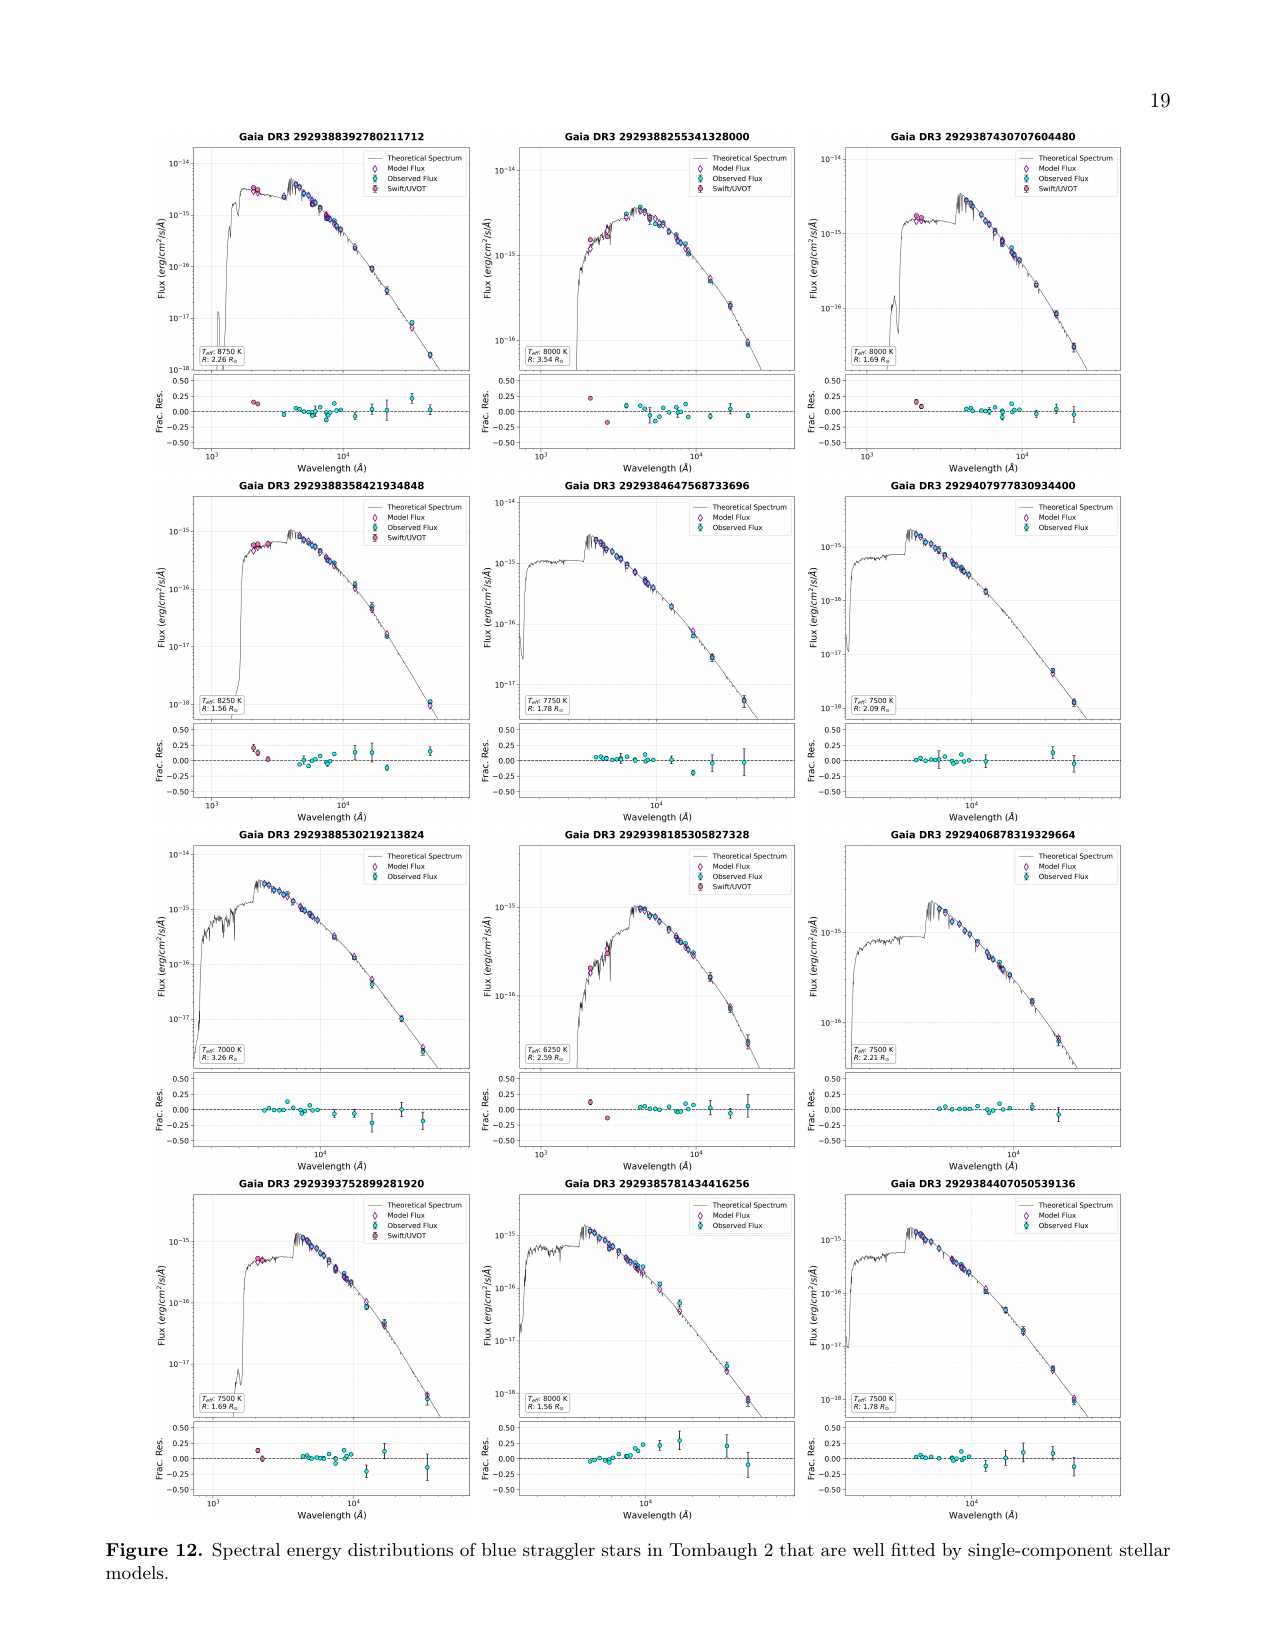}
    \caption{Spectral energy distributions of blue straggler stars in Tombaugh 2 that are well fitted by single-component stellar models.}
\end{figure*}

\begin{figure*}[t]
    \centering
    \includegraphics[width=0.92\linewidth]{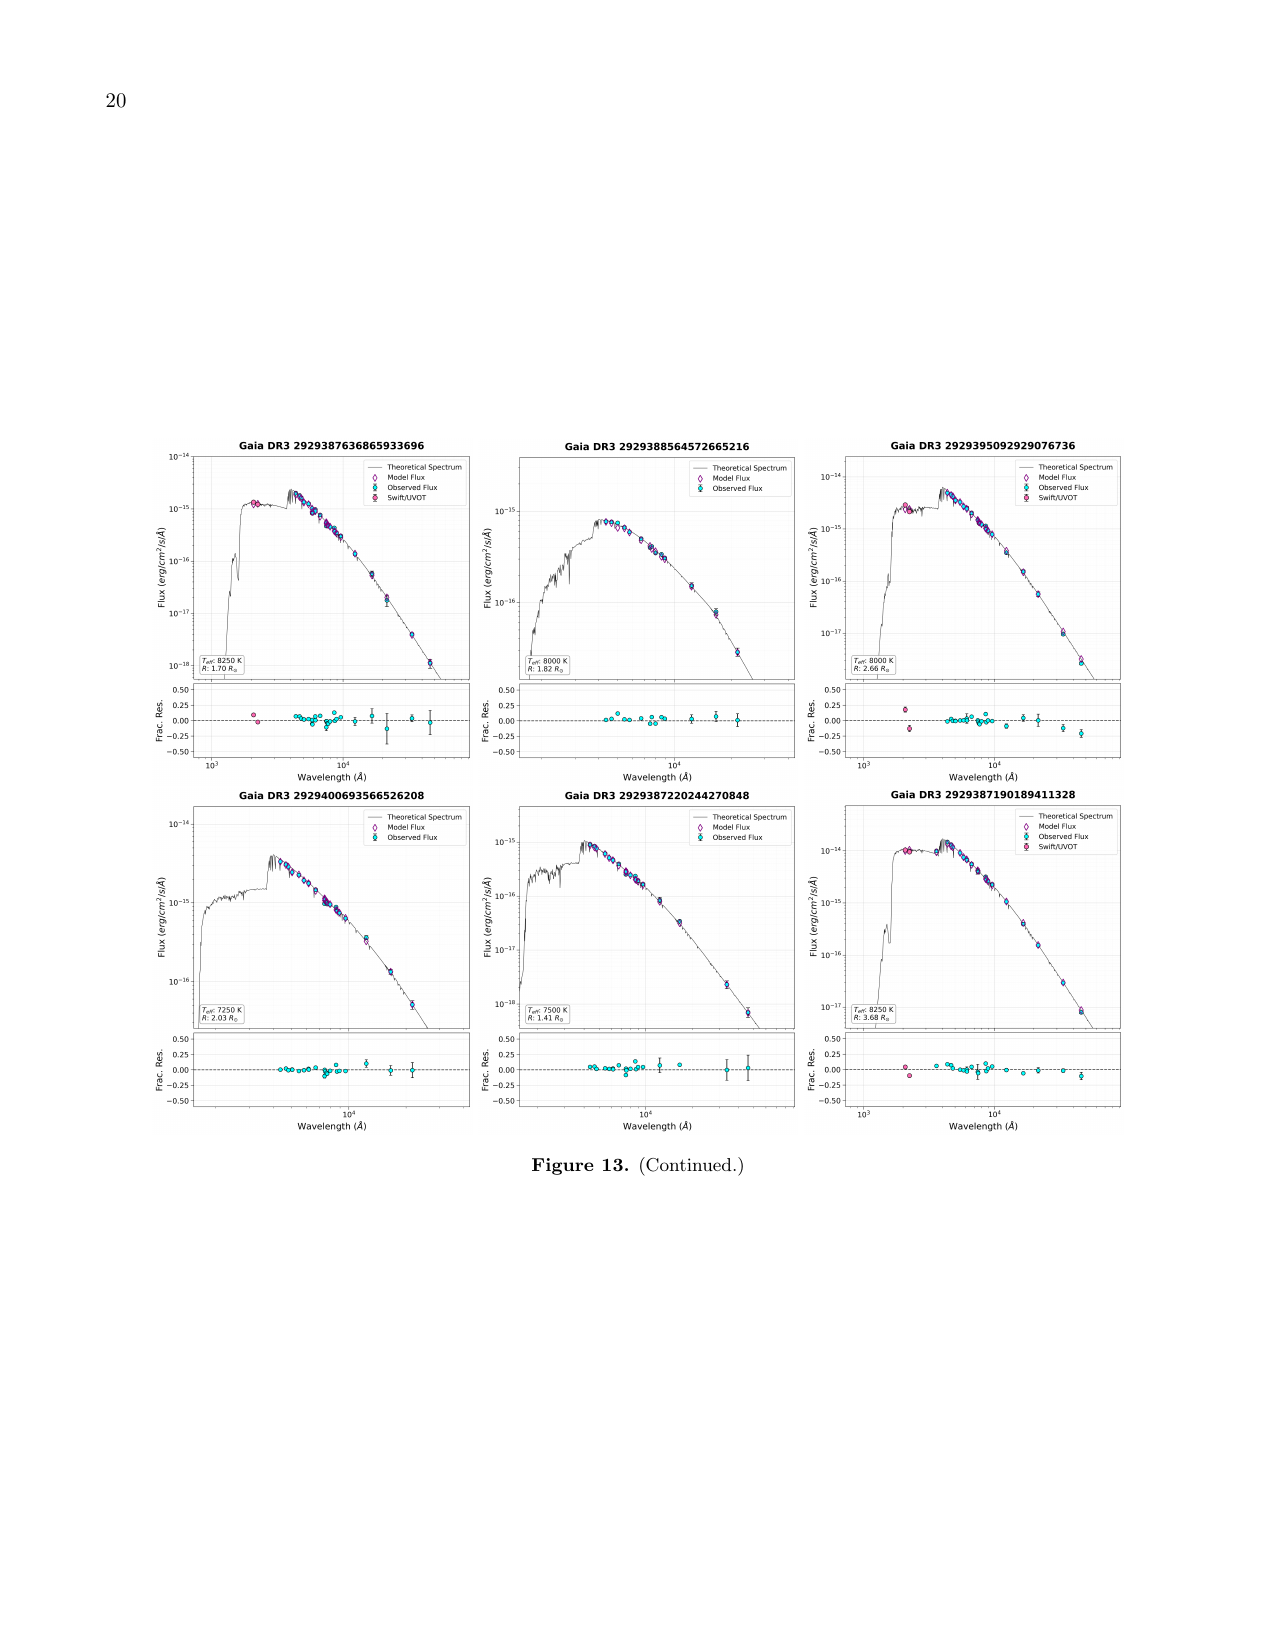}
    \caption{(Continued.)}
\end{figure*}

%\begin{figure*}
%    \centering
%    \includegraphics[width=0.3\linewidth]{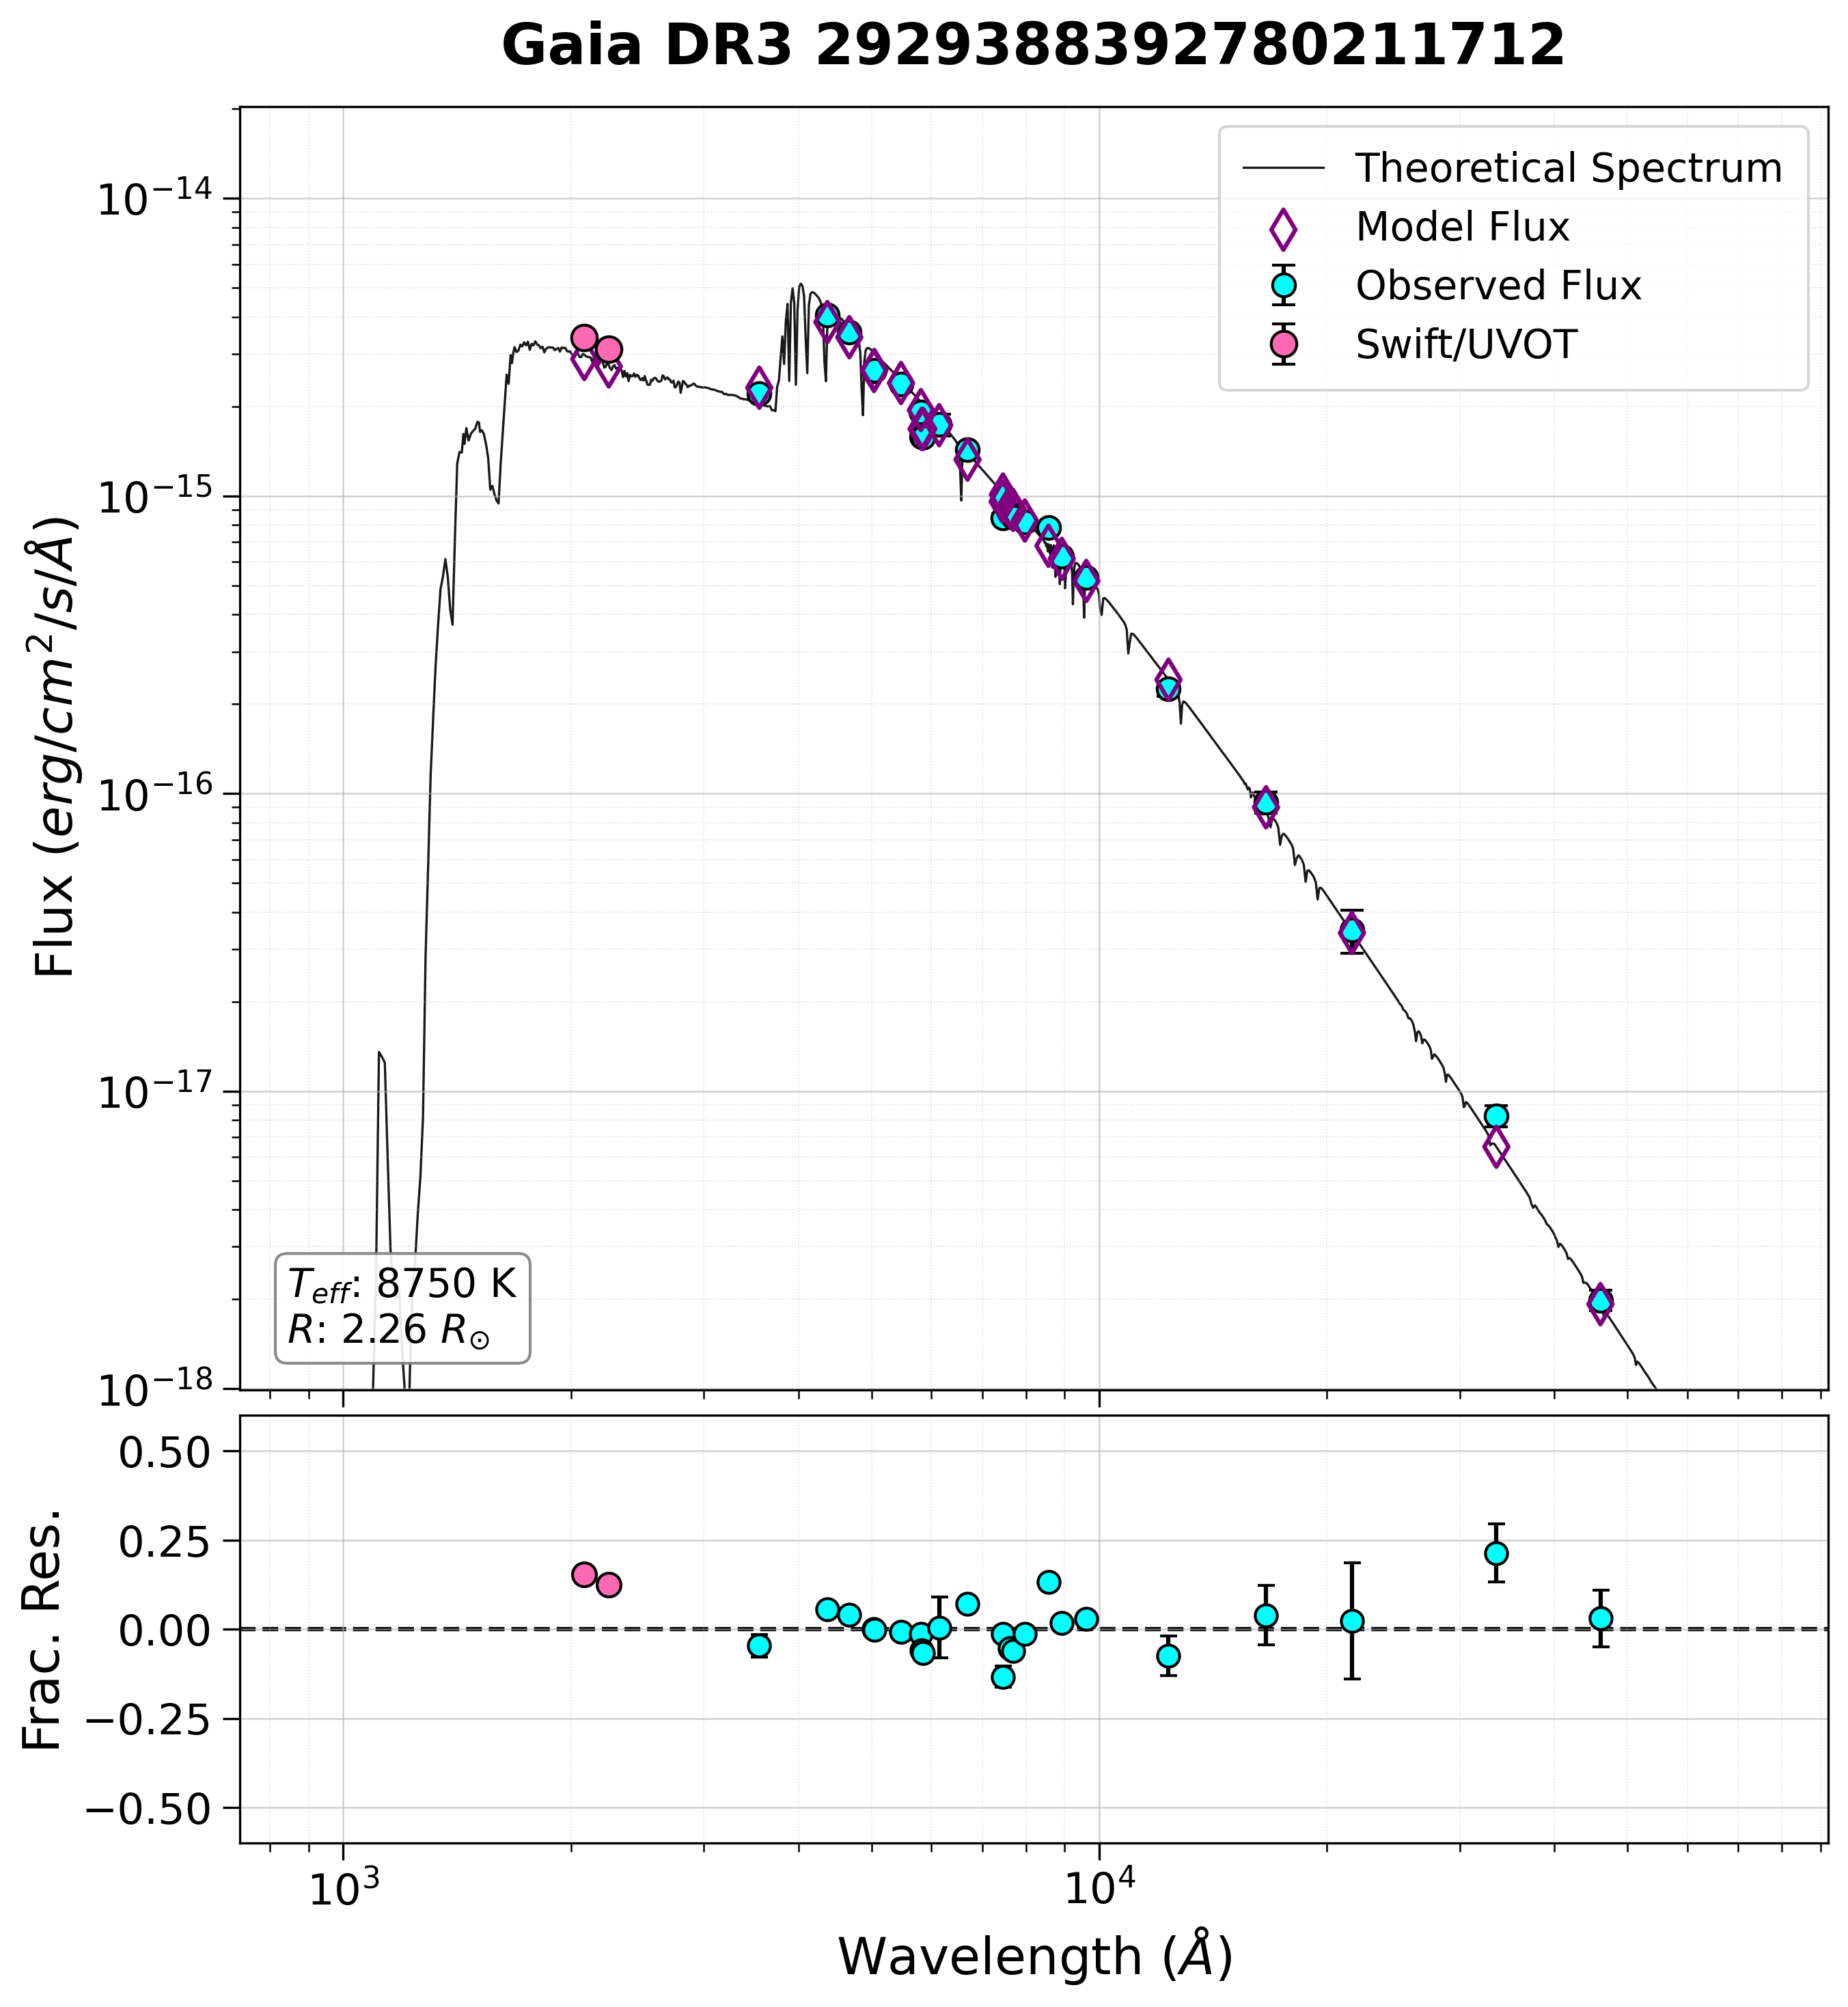}
%    \includegraphics[width=0.3\linewidth]{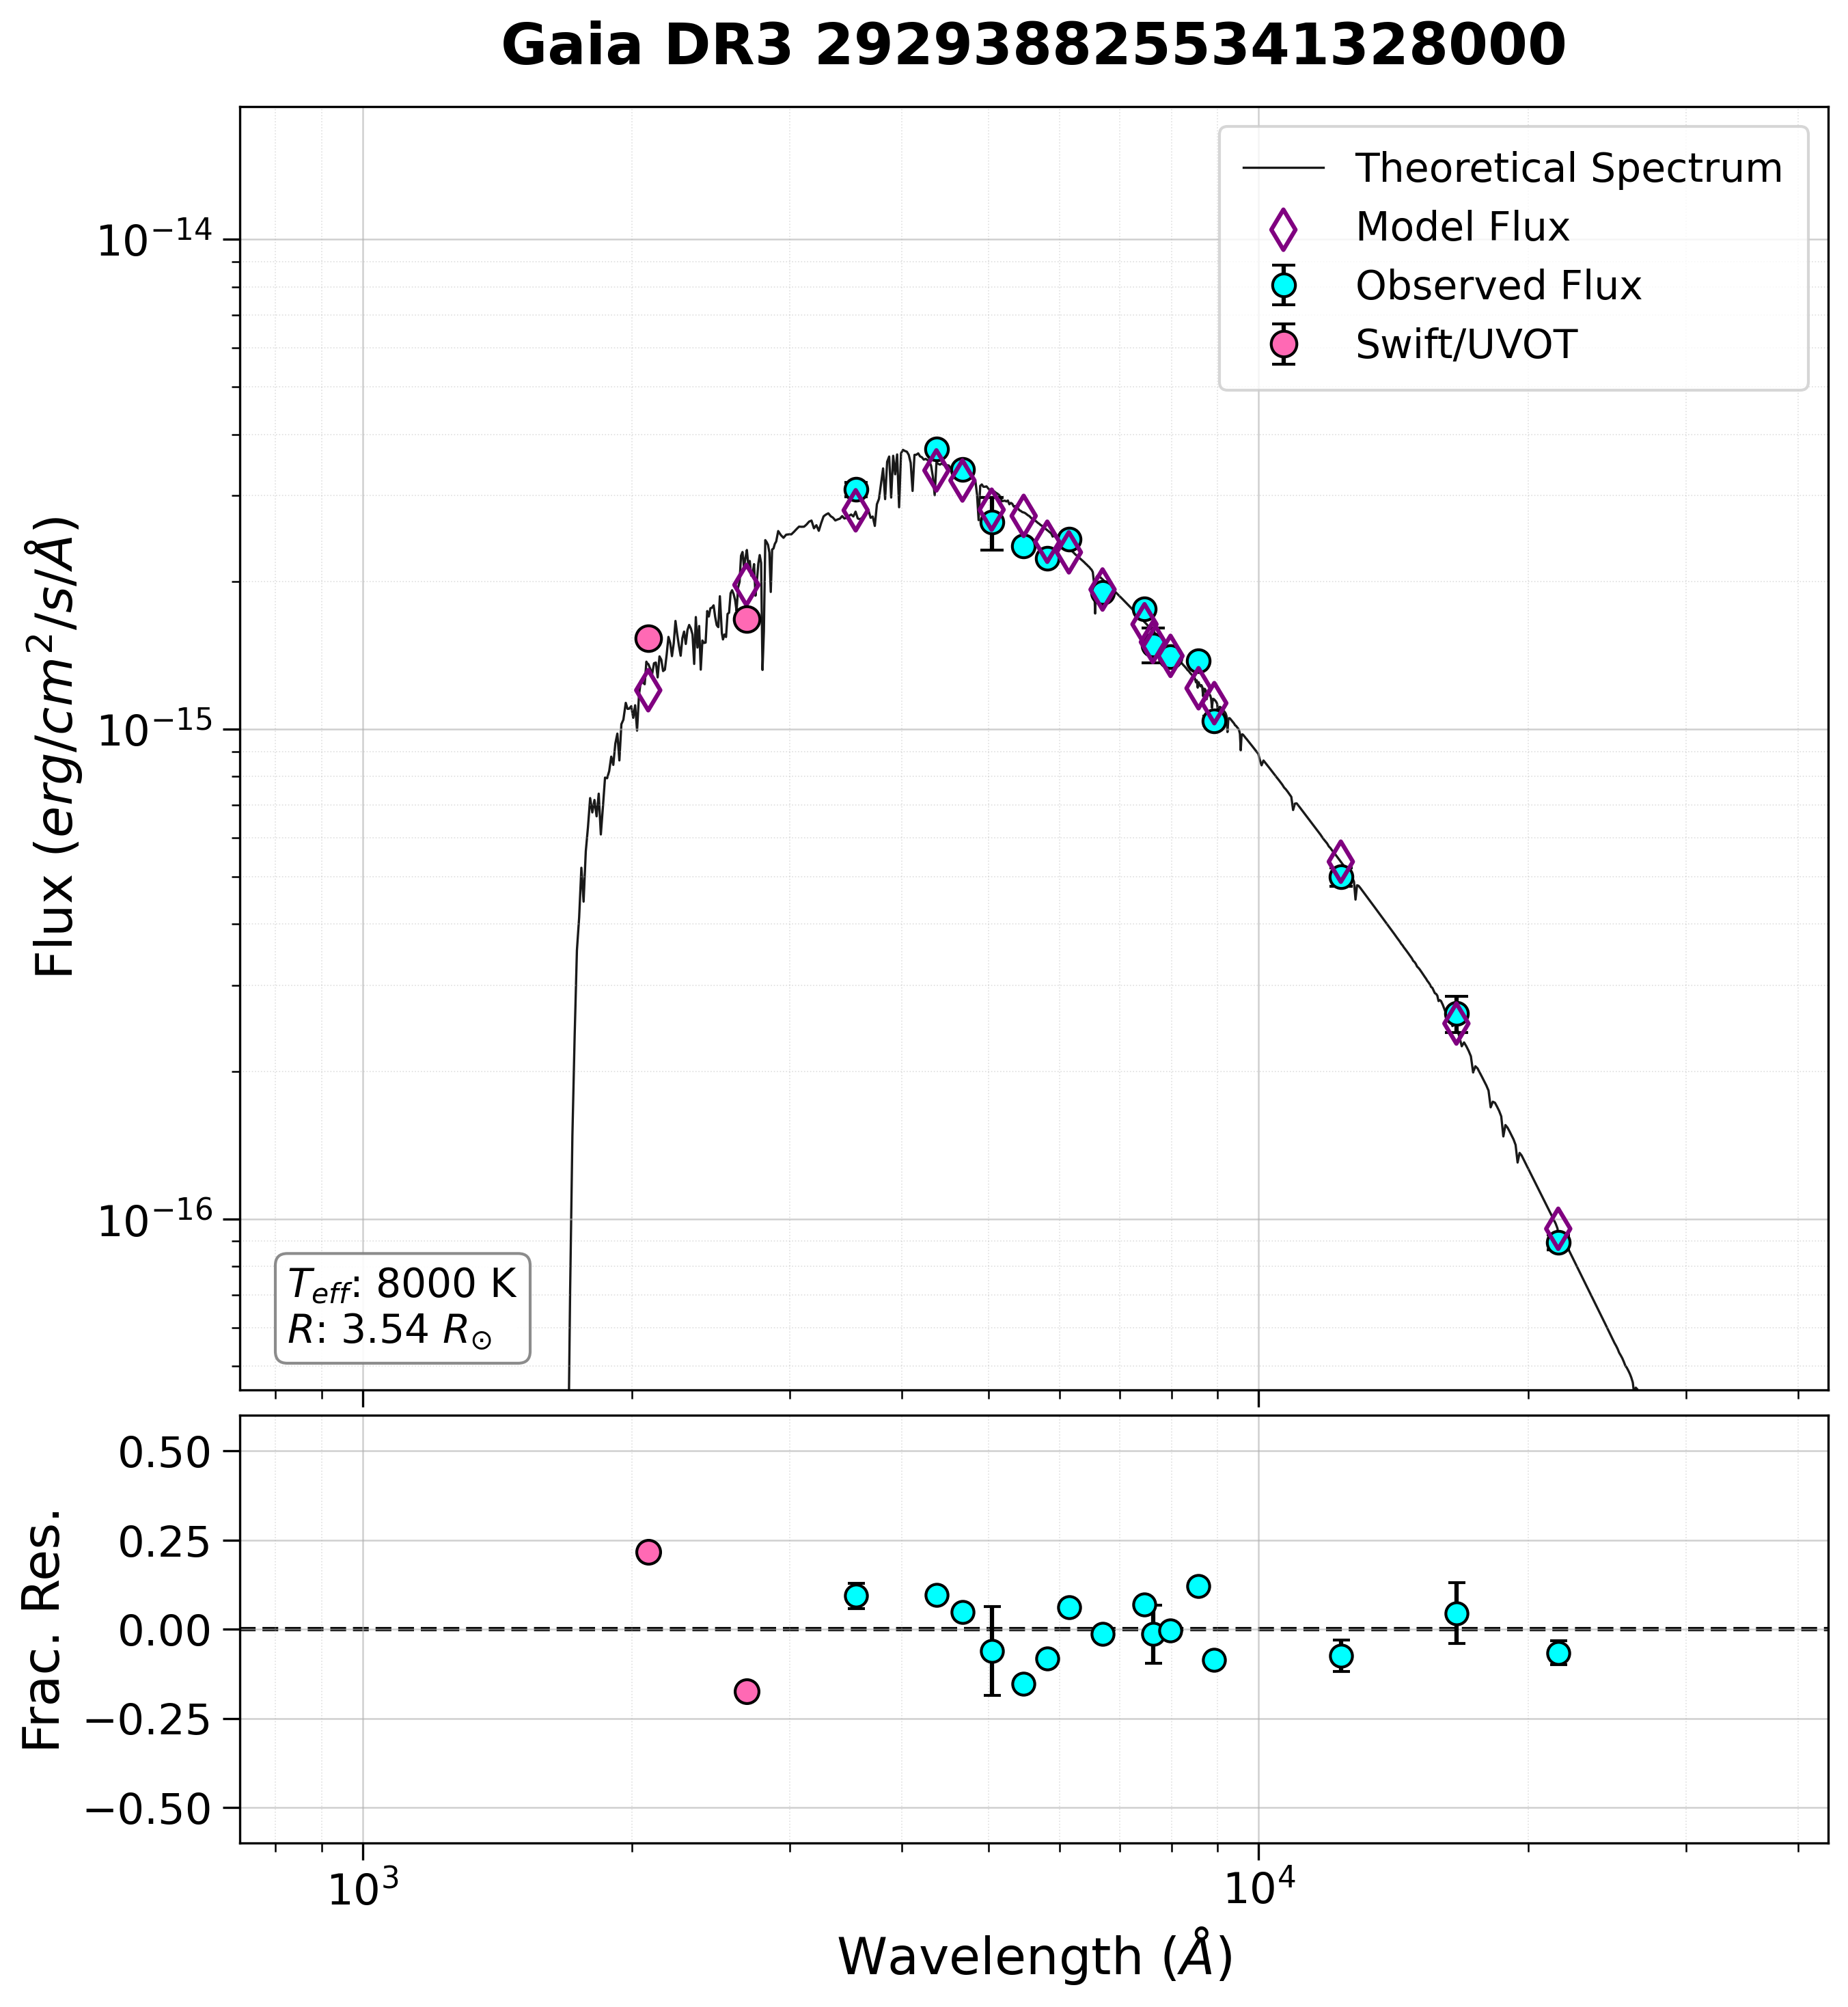}
%    \includegraphics[width=0.3\linewidth]{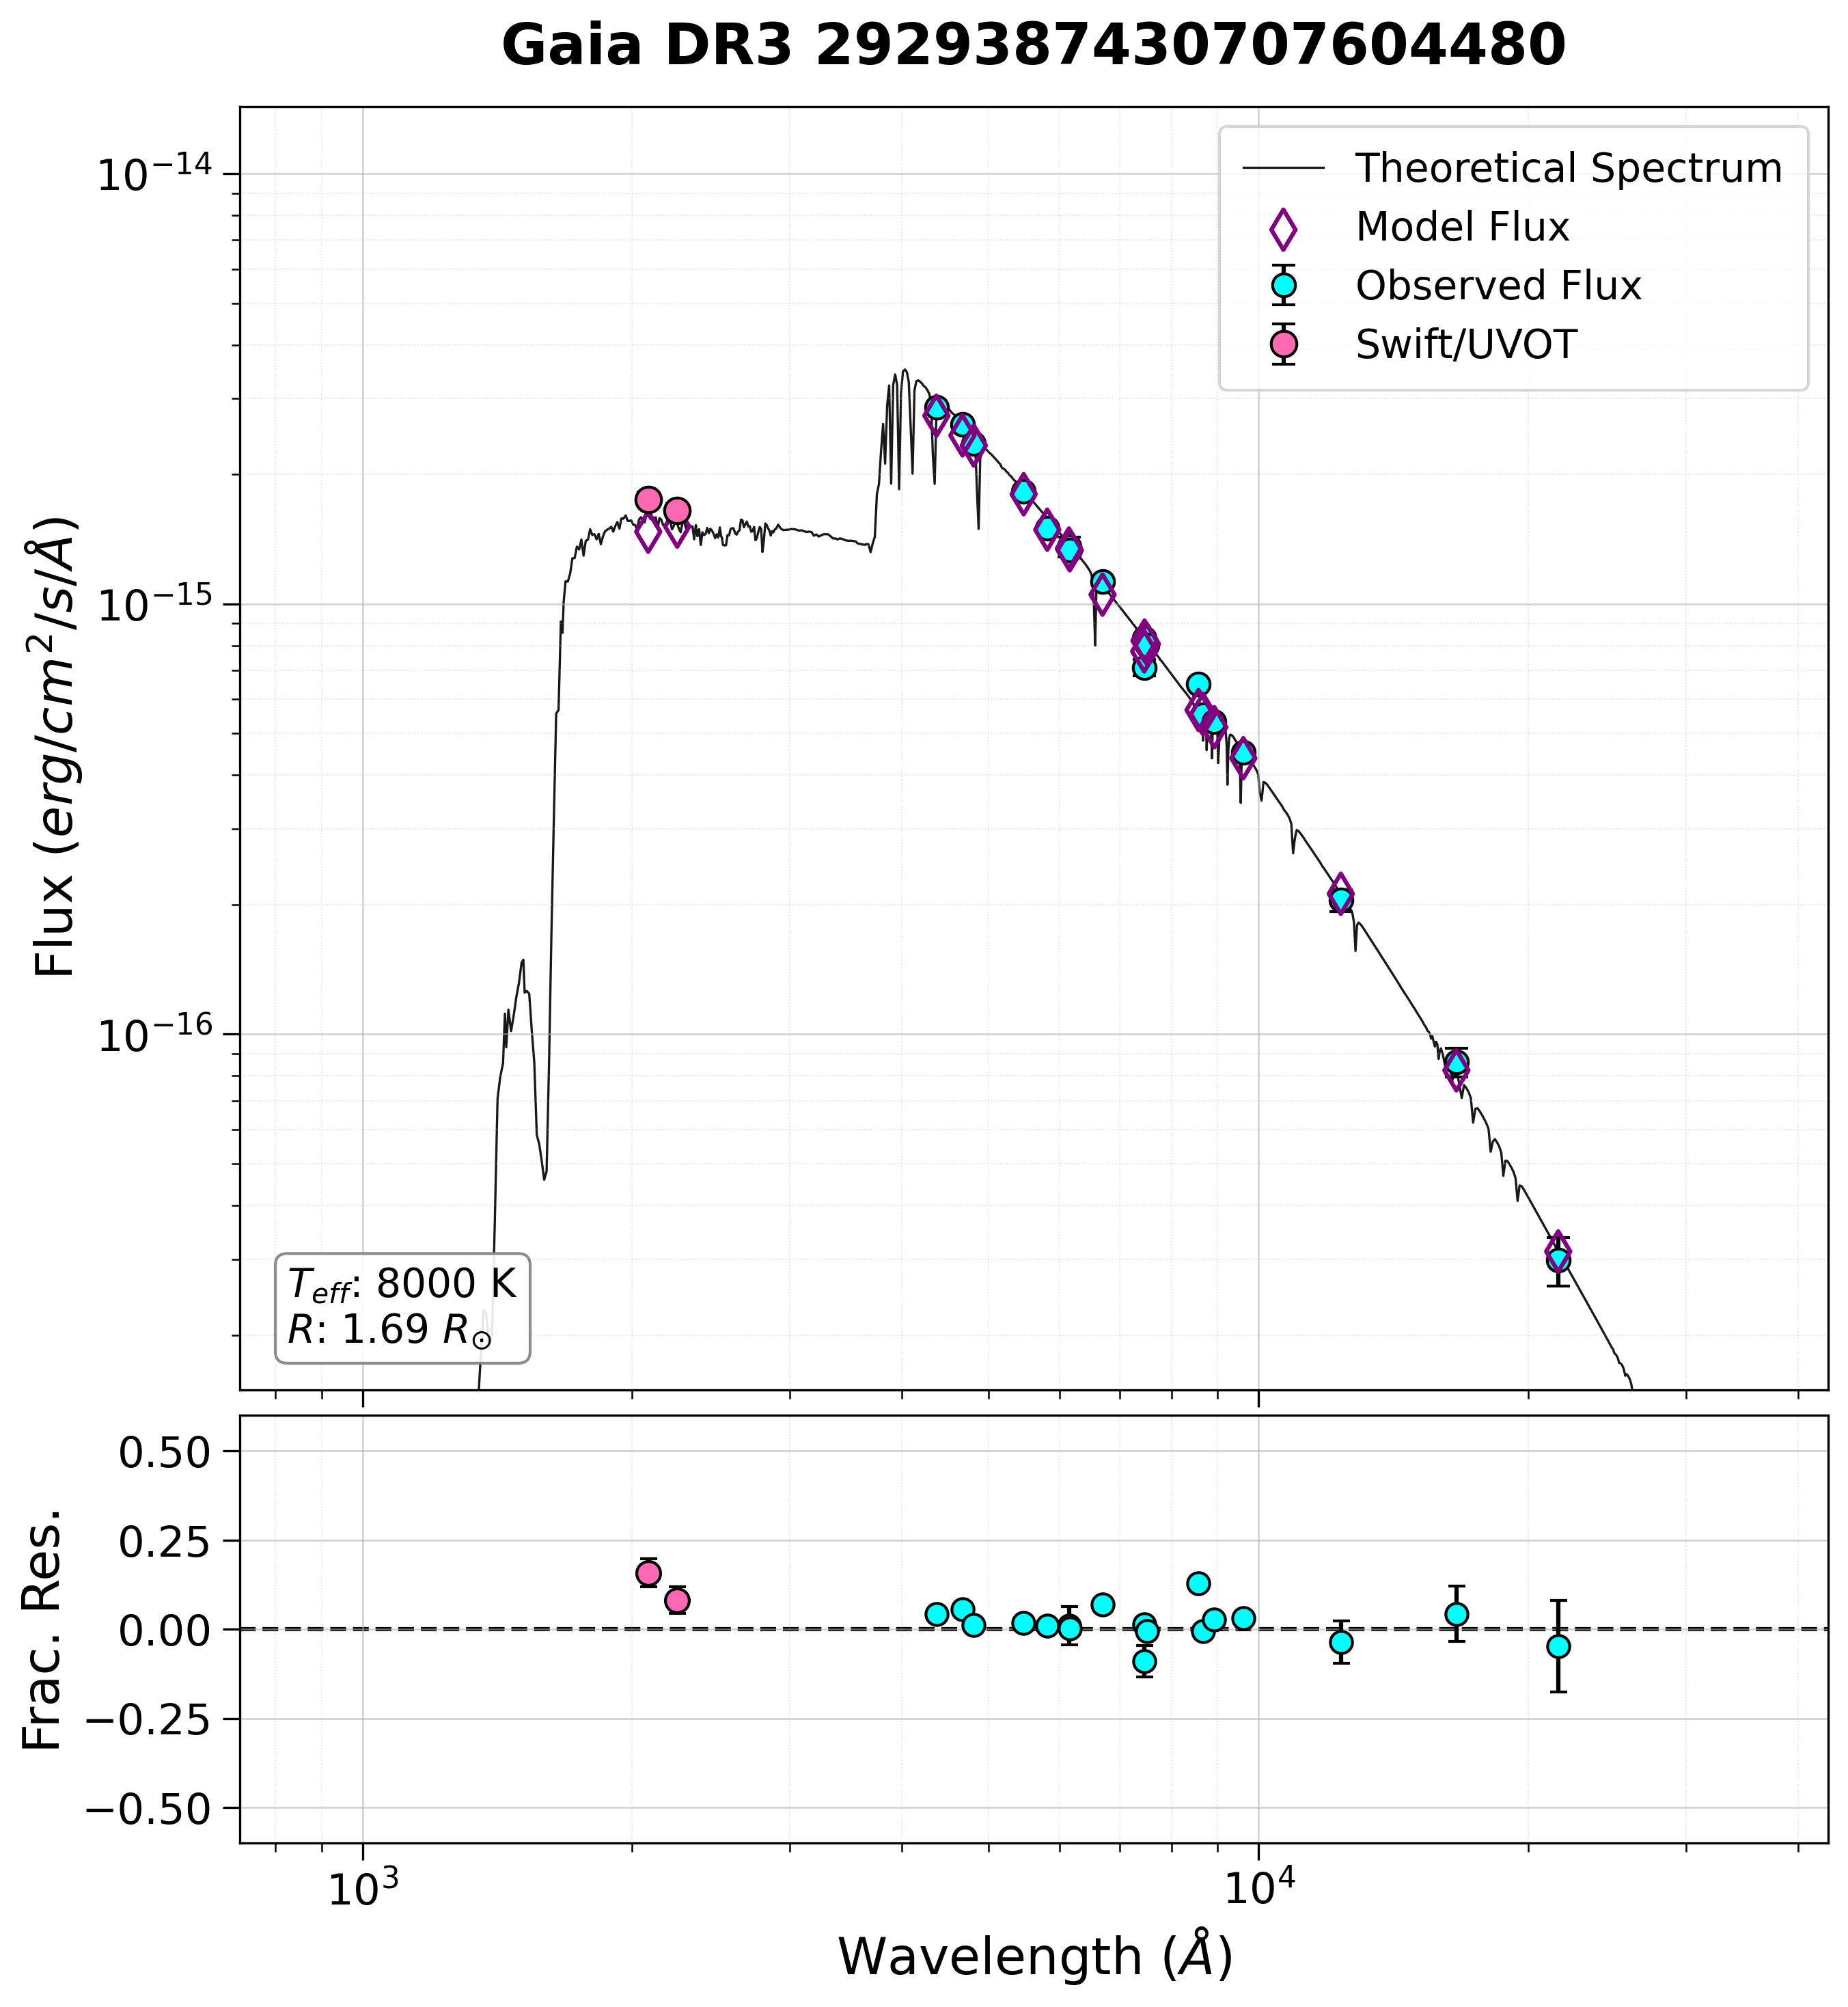}\\
%    \includegraphics[width=0.3\linewidth]{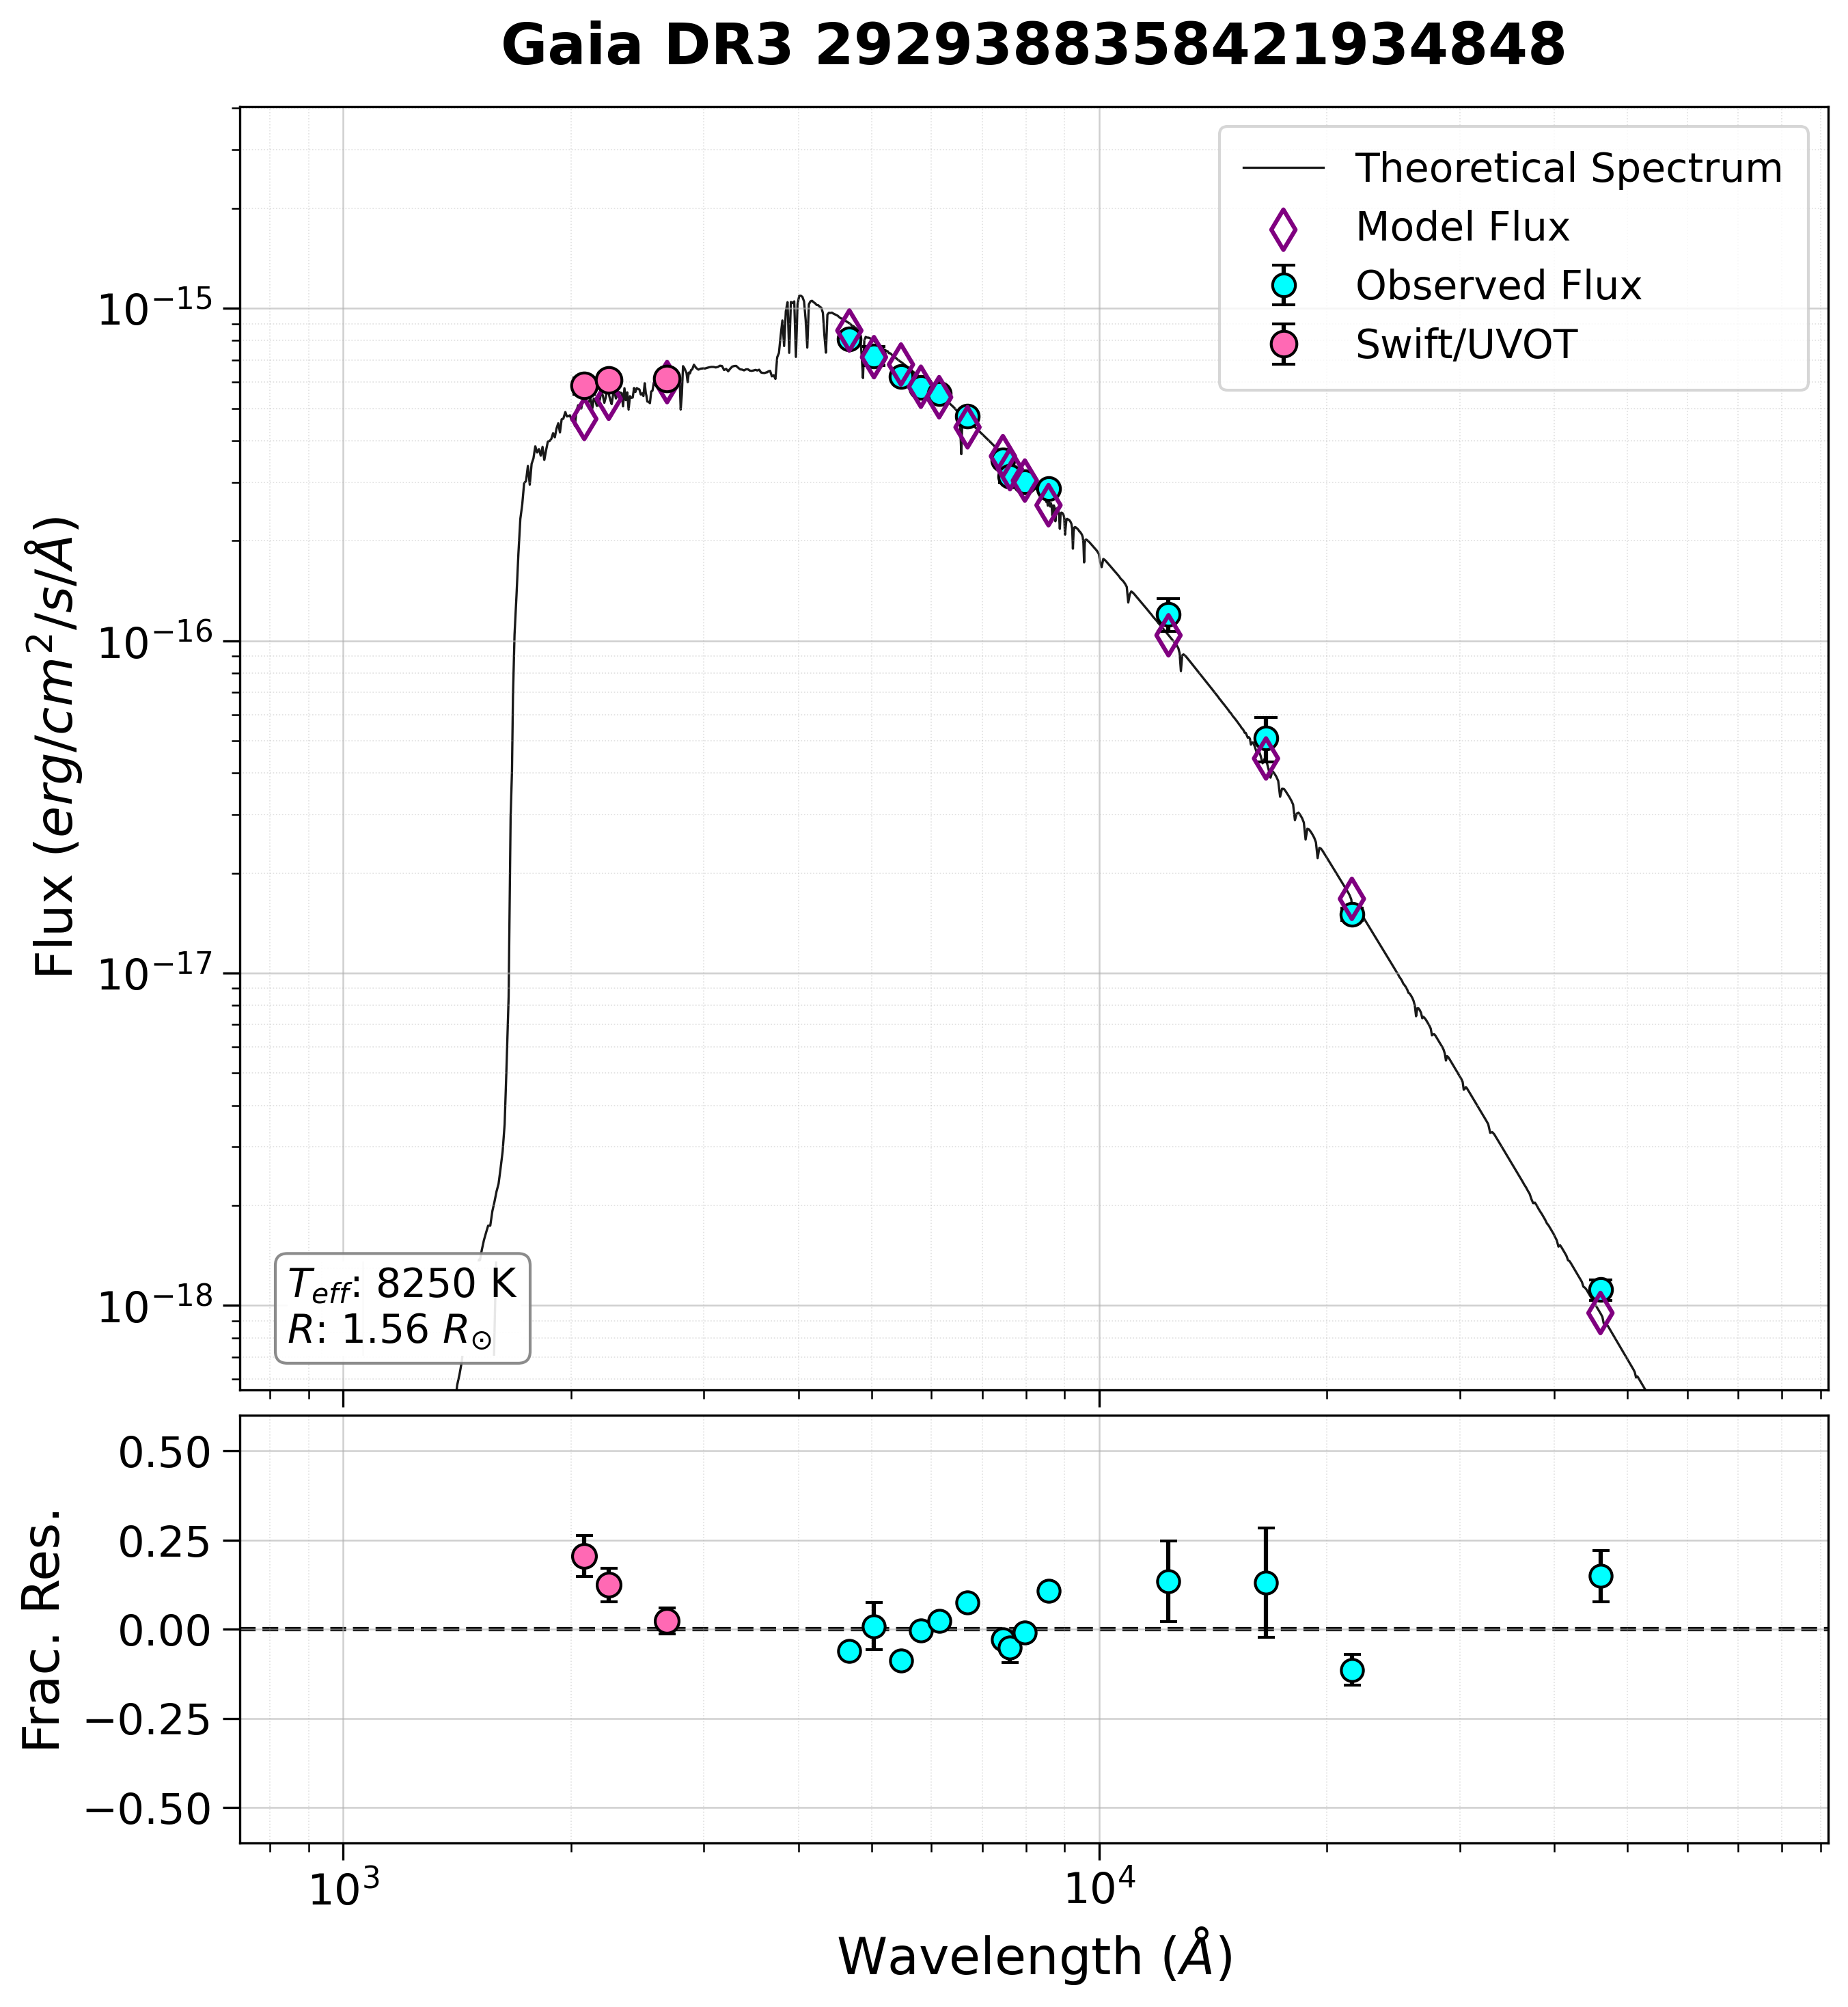}
%    \includegraphics[width=0.3\linewidth]{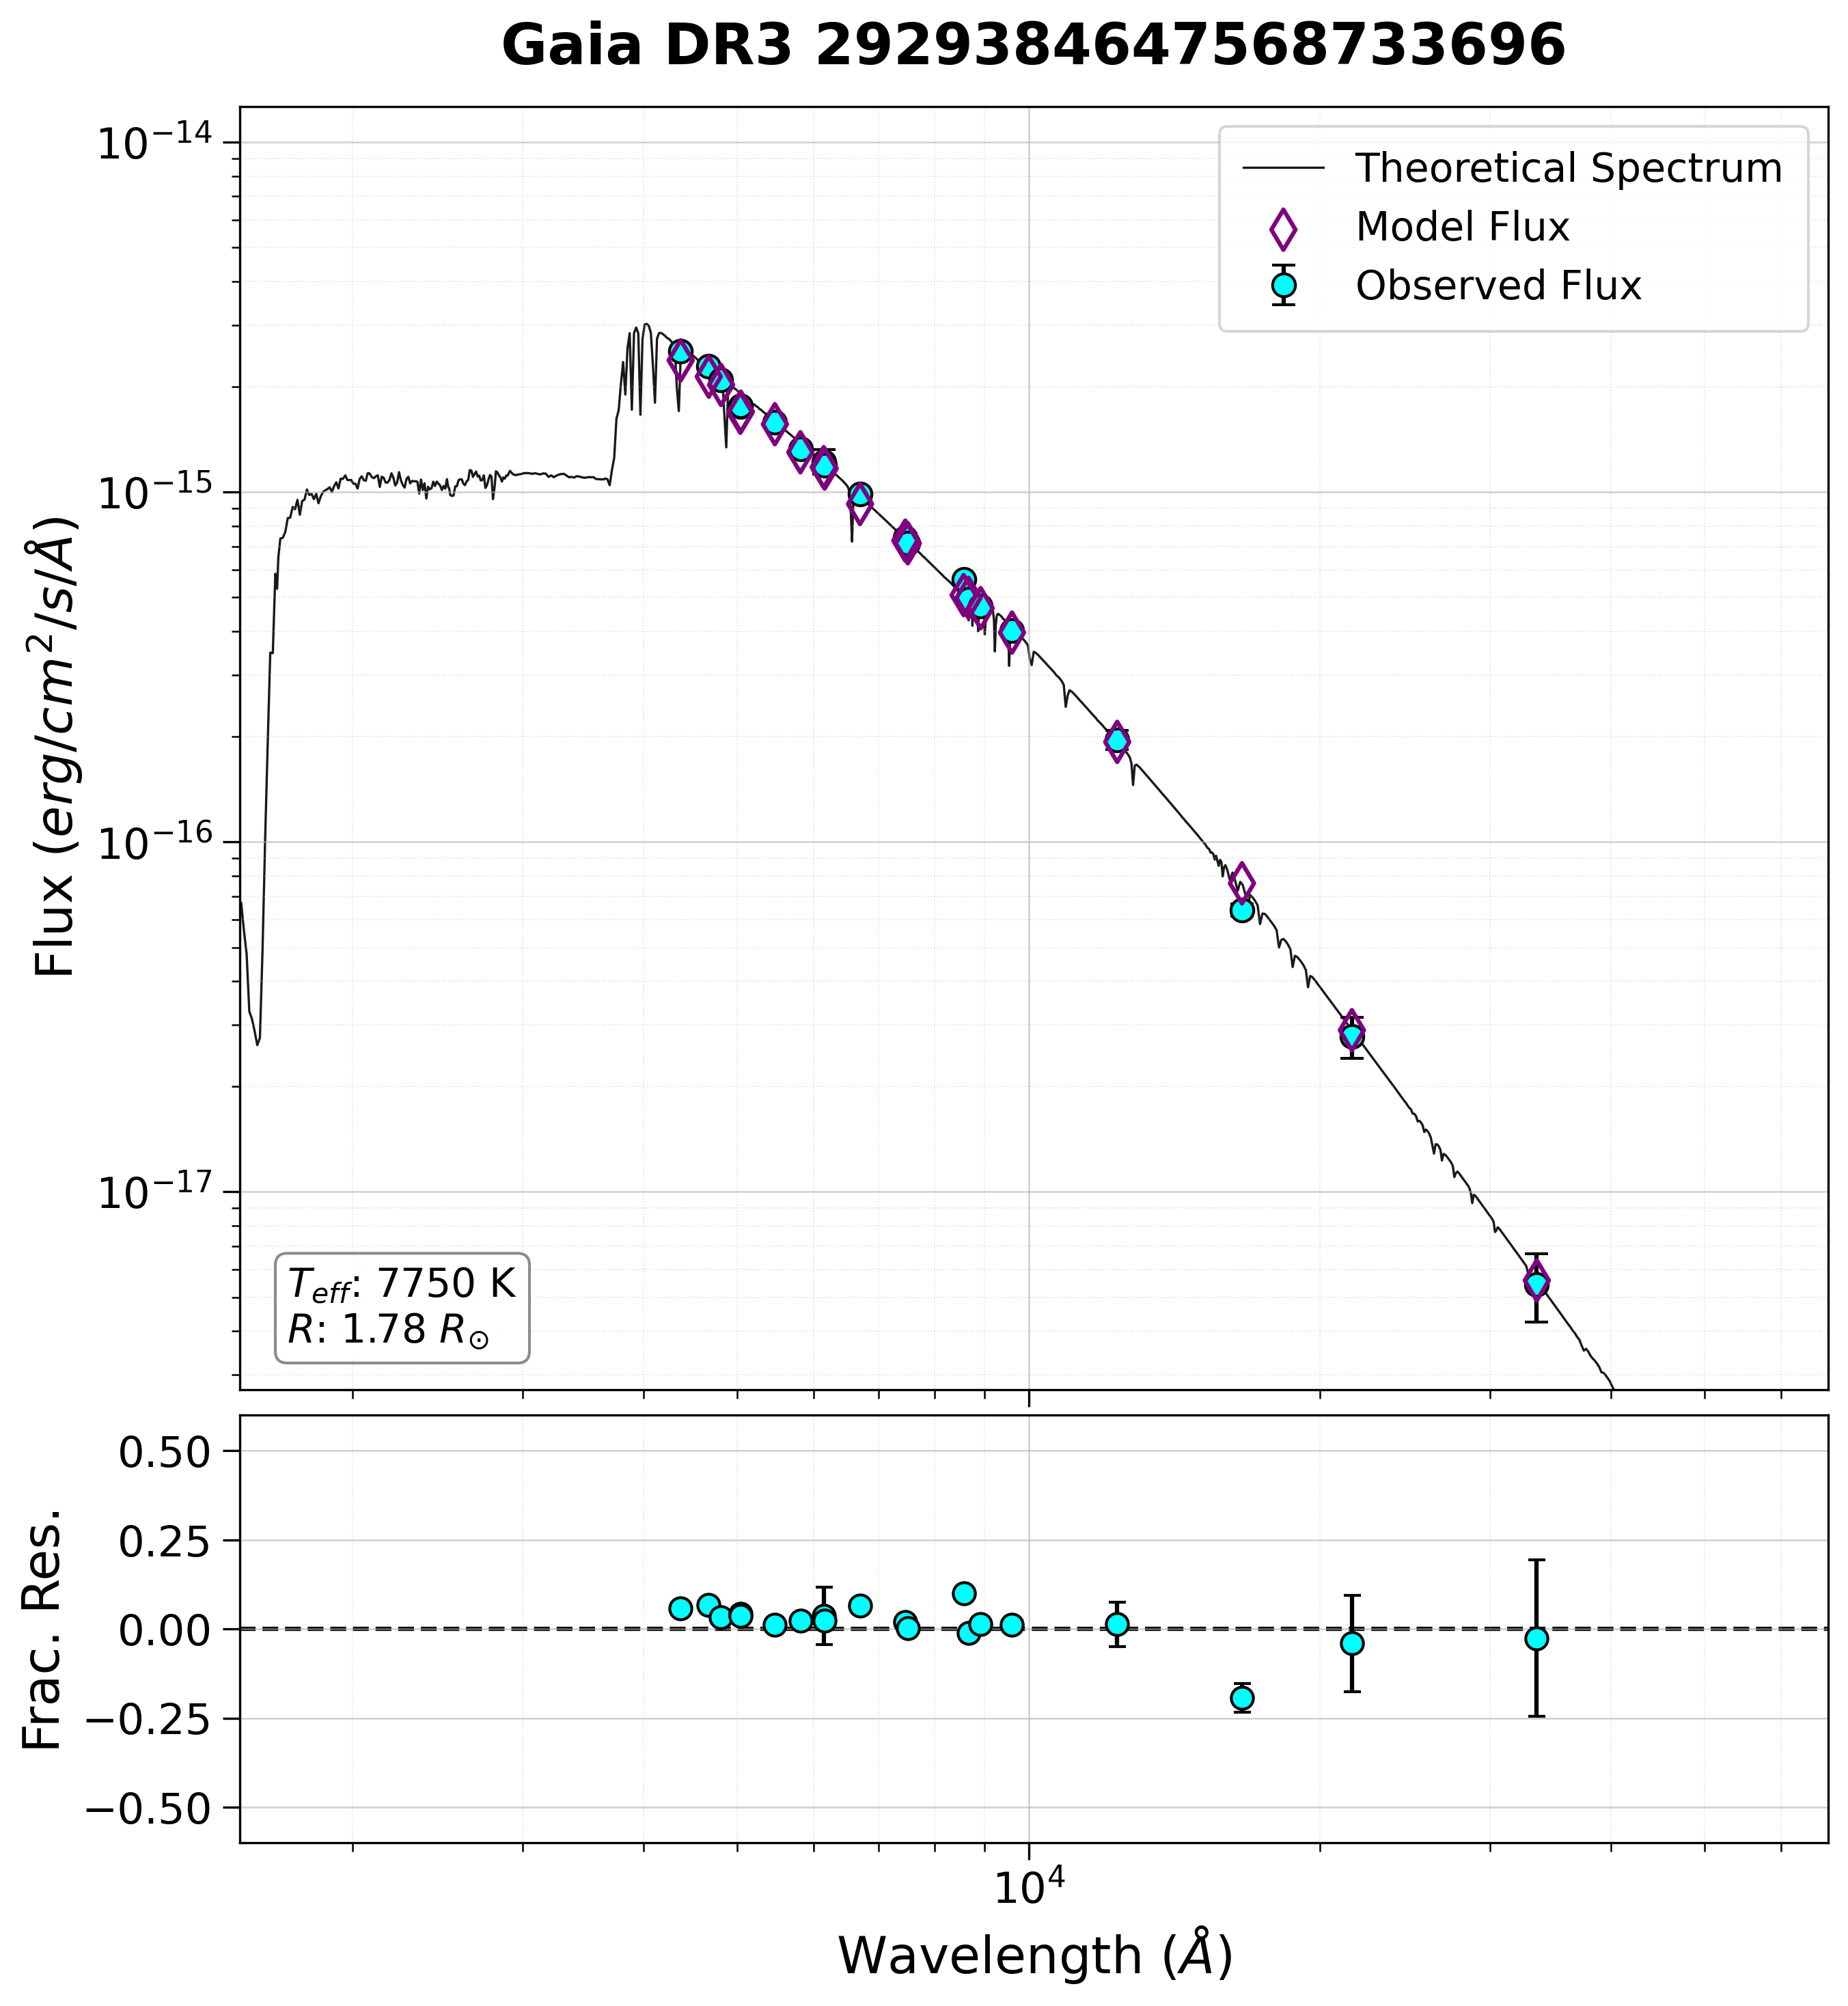}
%    \includegraphics[width=0.3\linewidth]{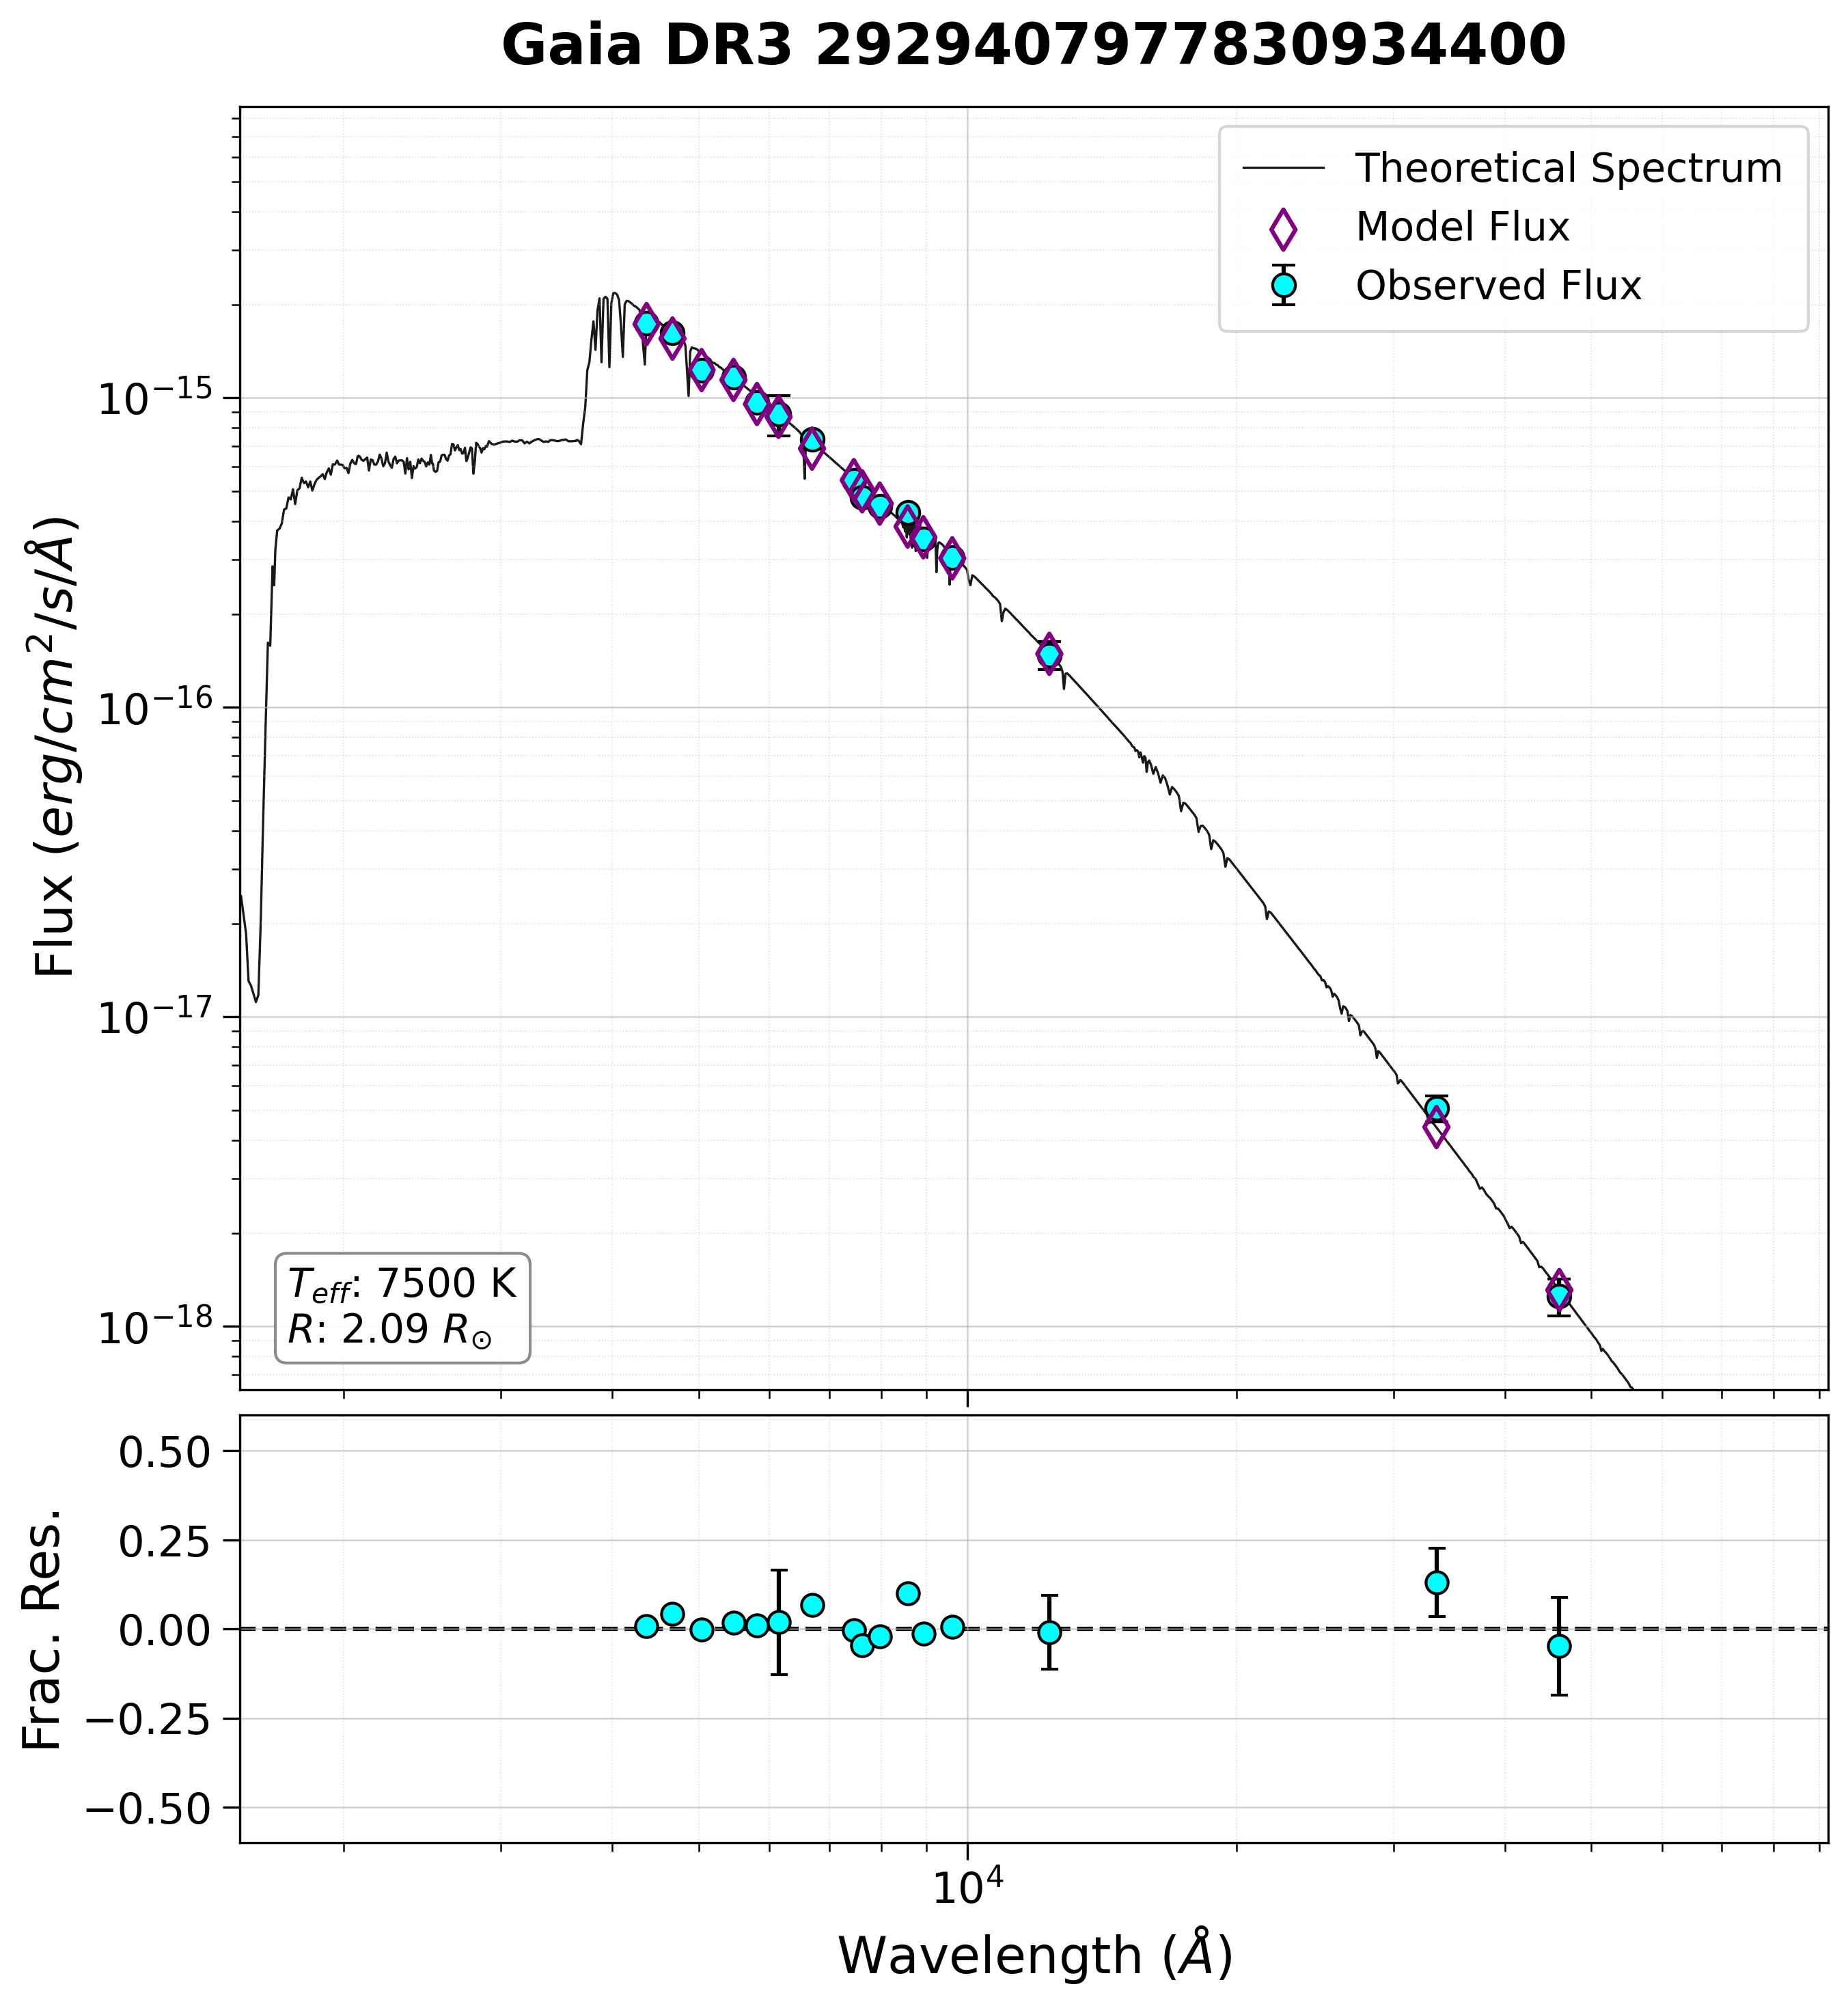}\\
%    \includegraphics[width=0.3\linewidth]{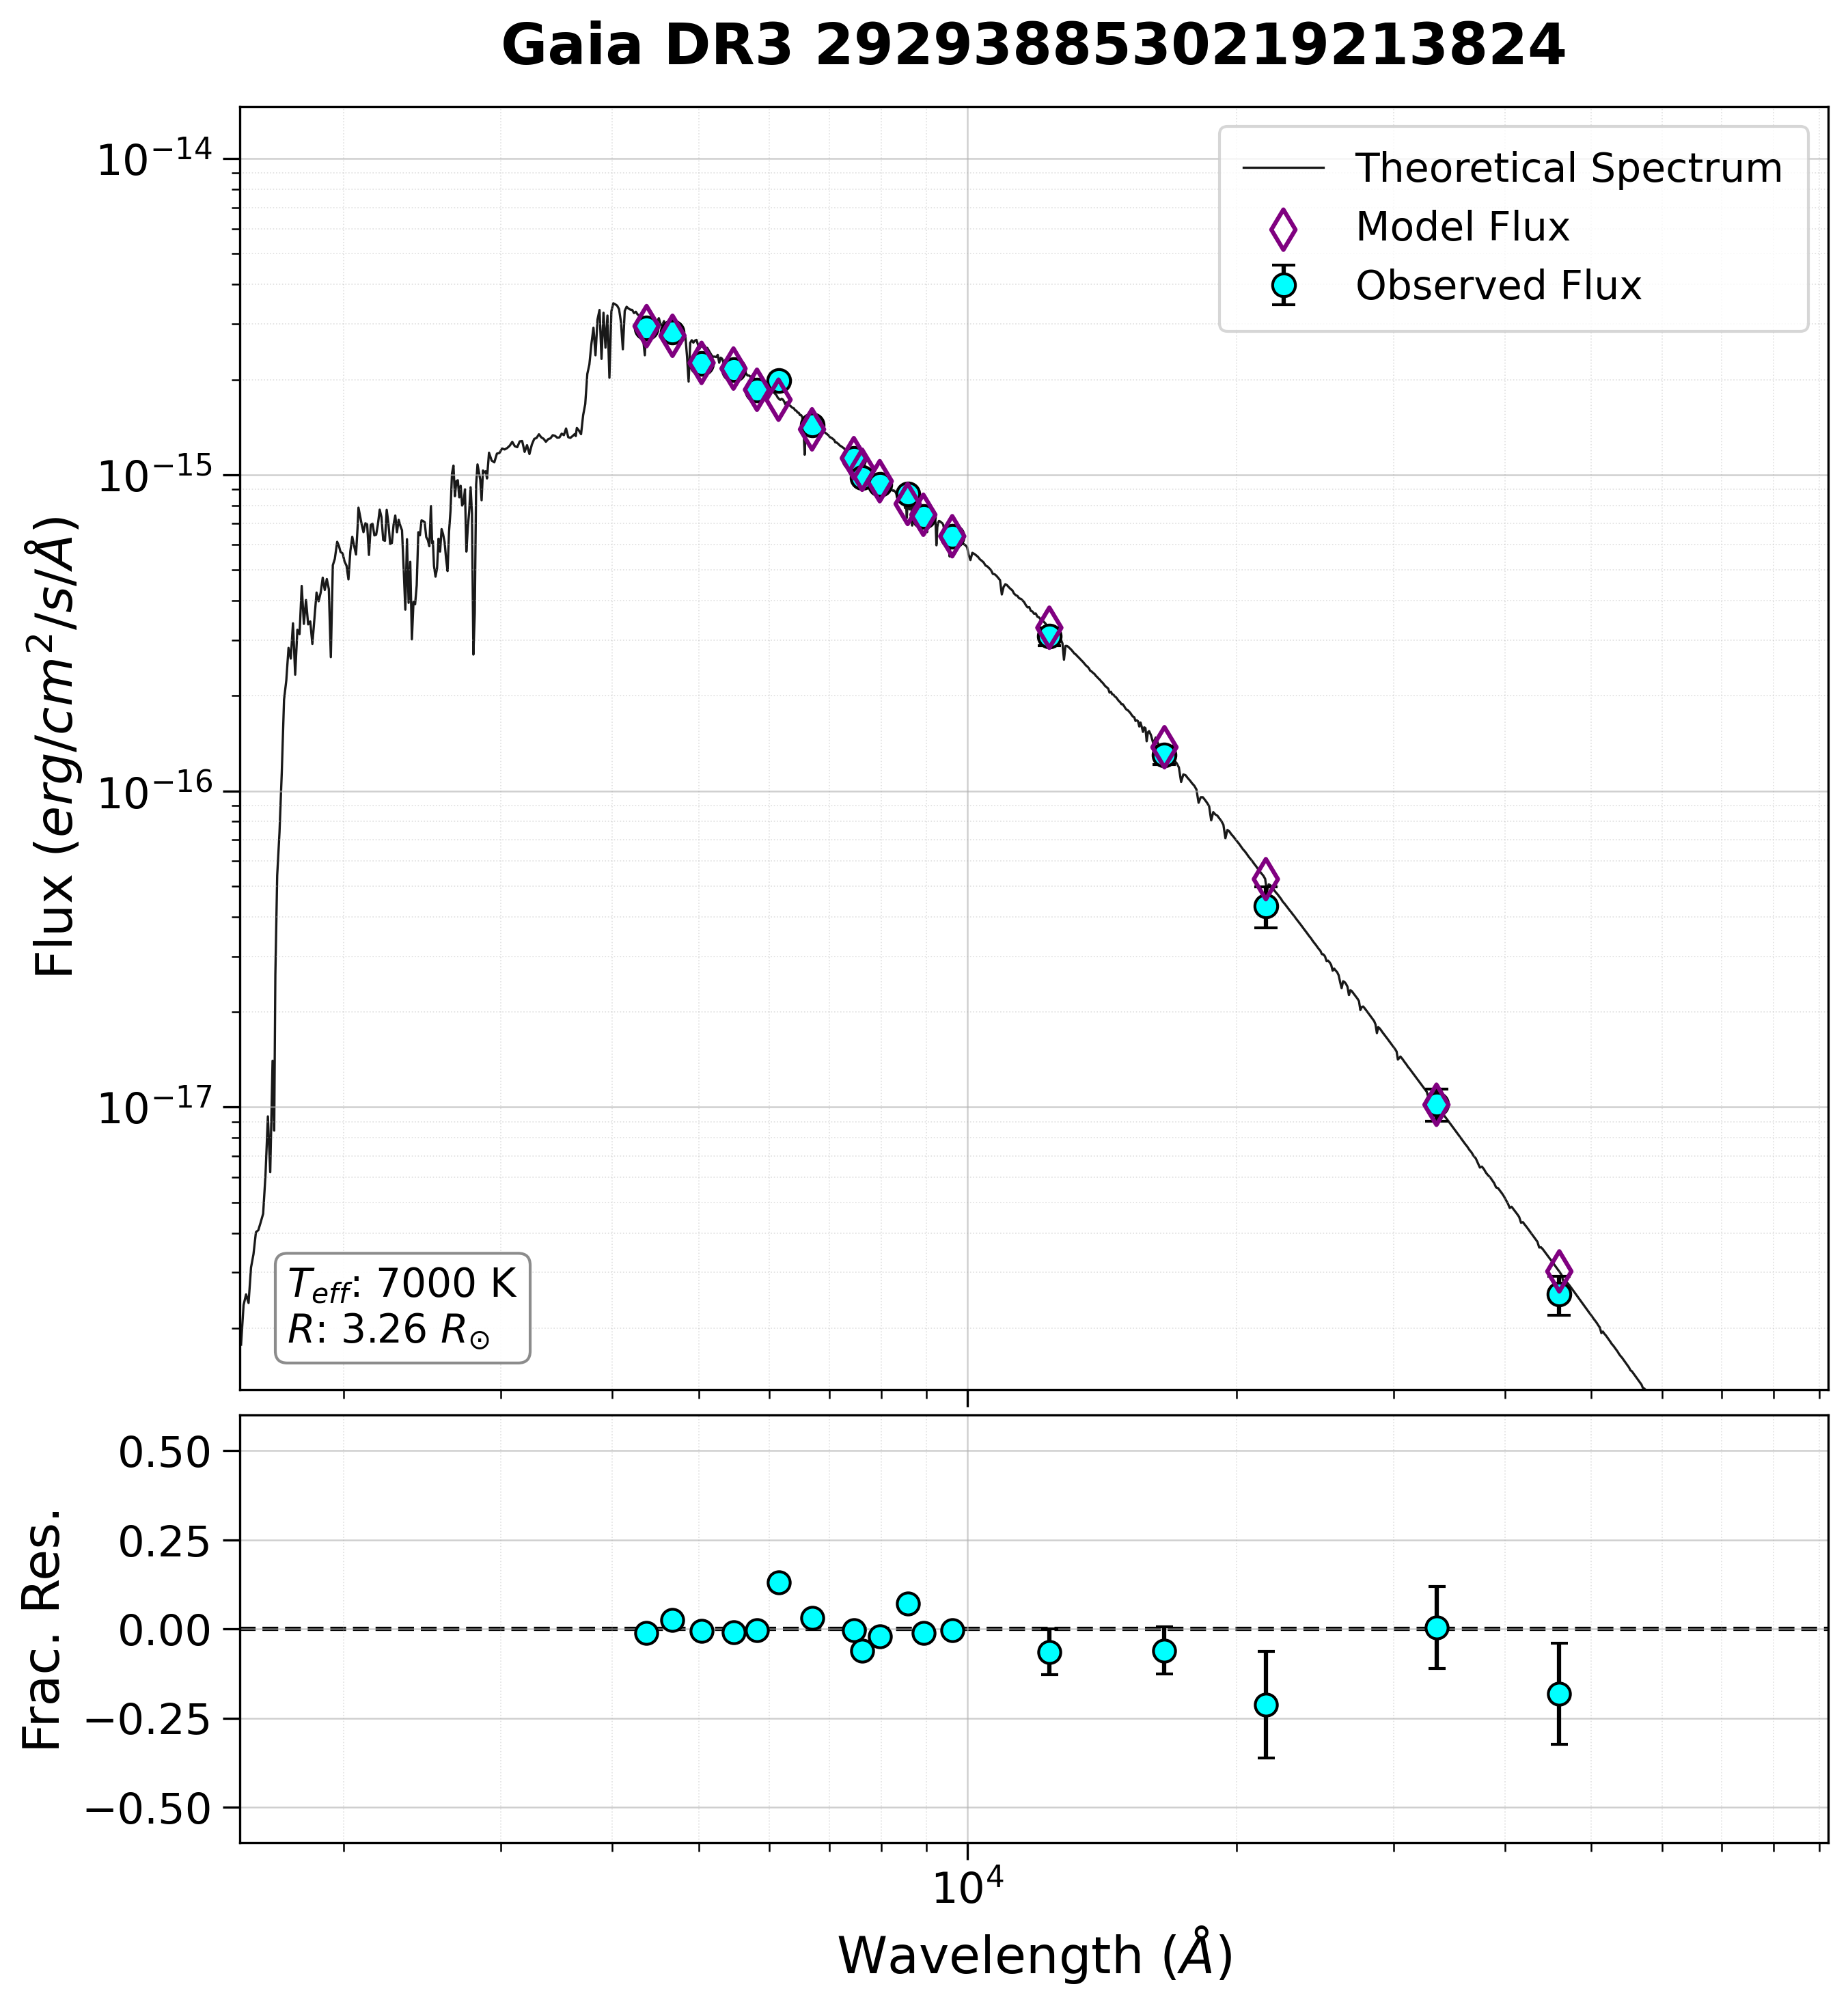}
%    \includegraphics[width=0.3\linewidth]{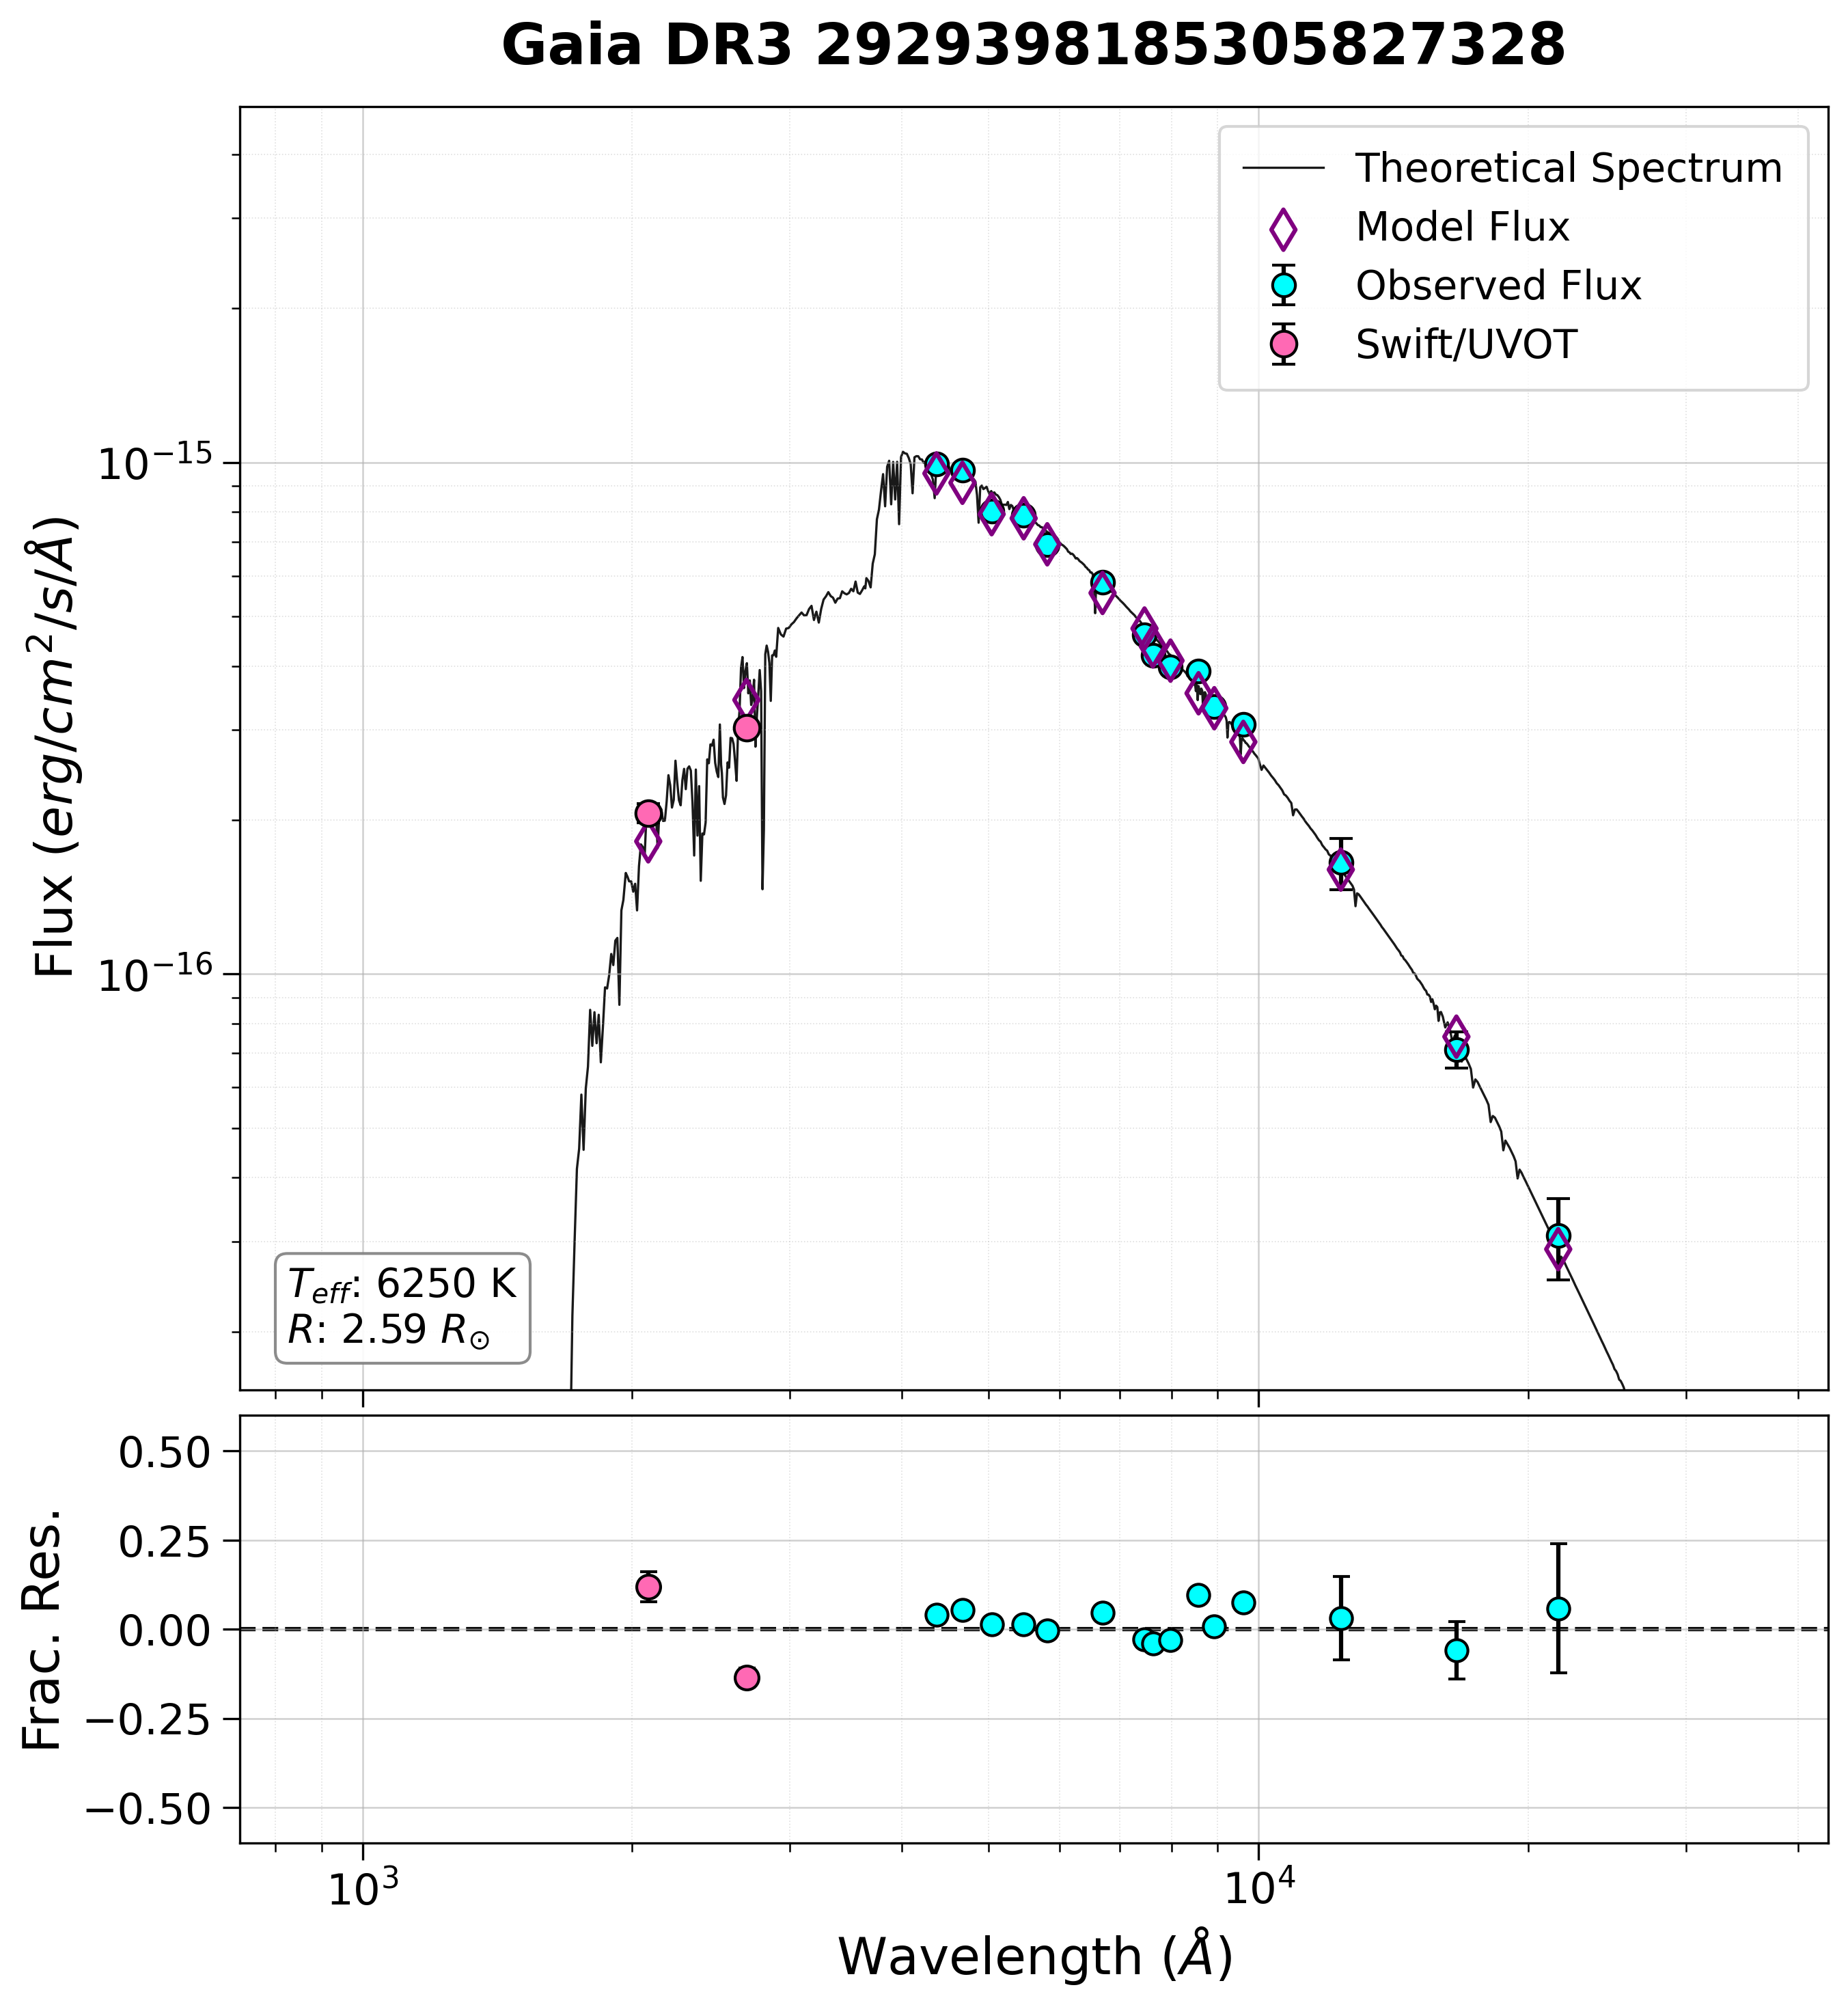}
%    \includegraphics[width=0.3\linewidth]{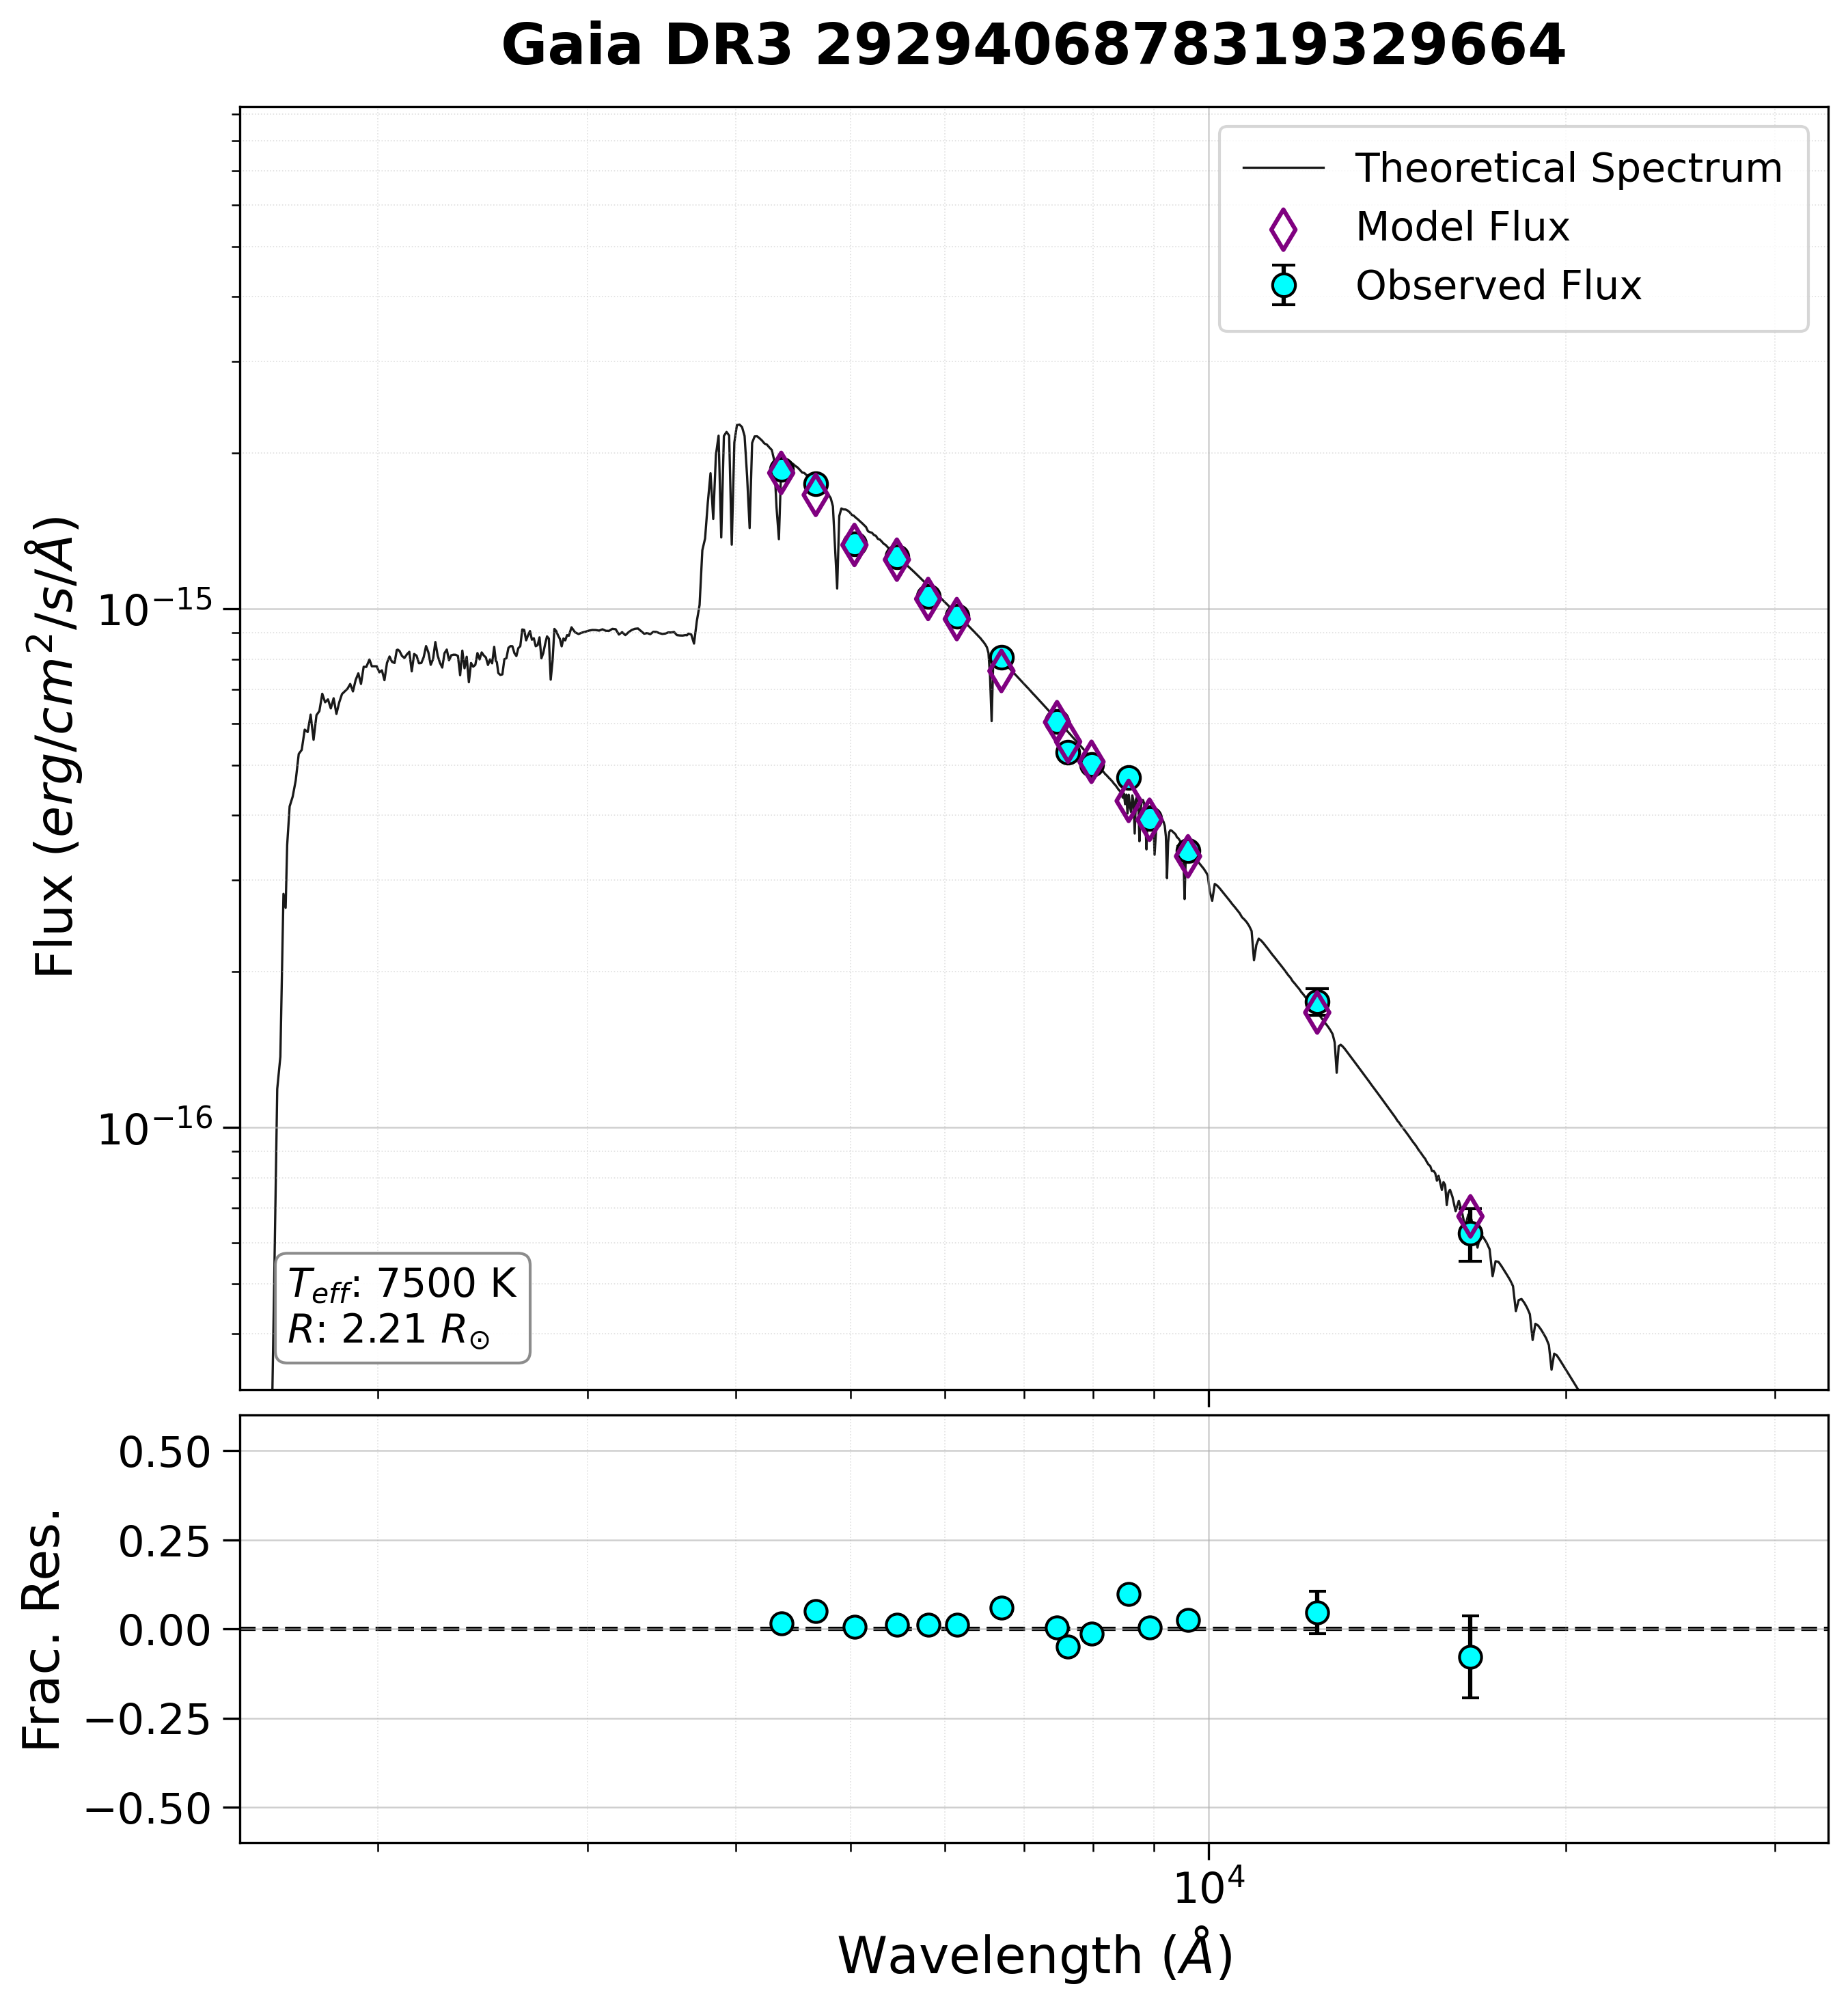}\\
%    \includegraphics[width=0.3\linewidth]{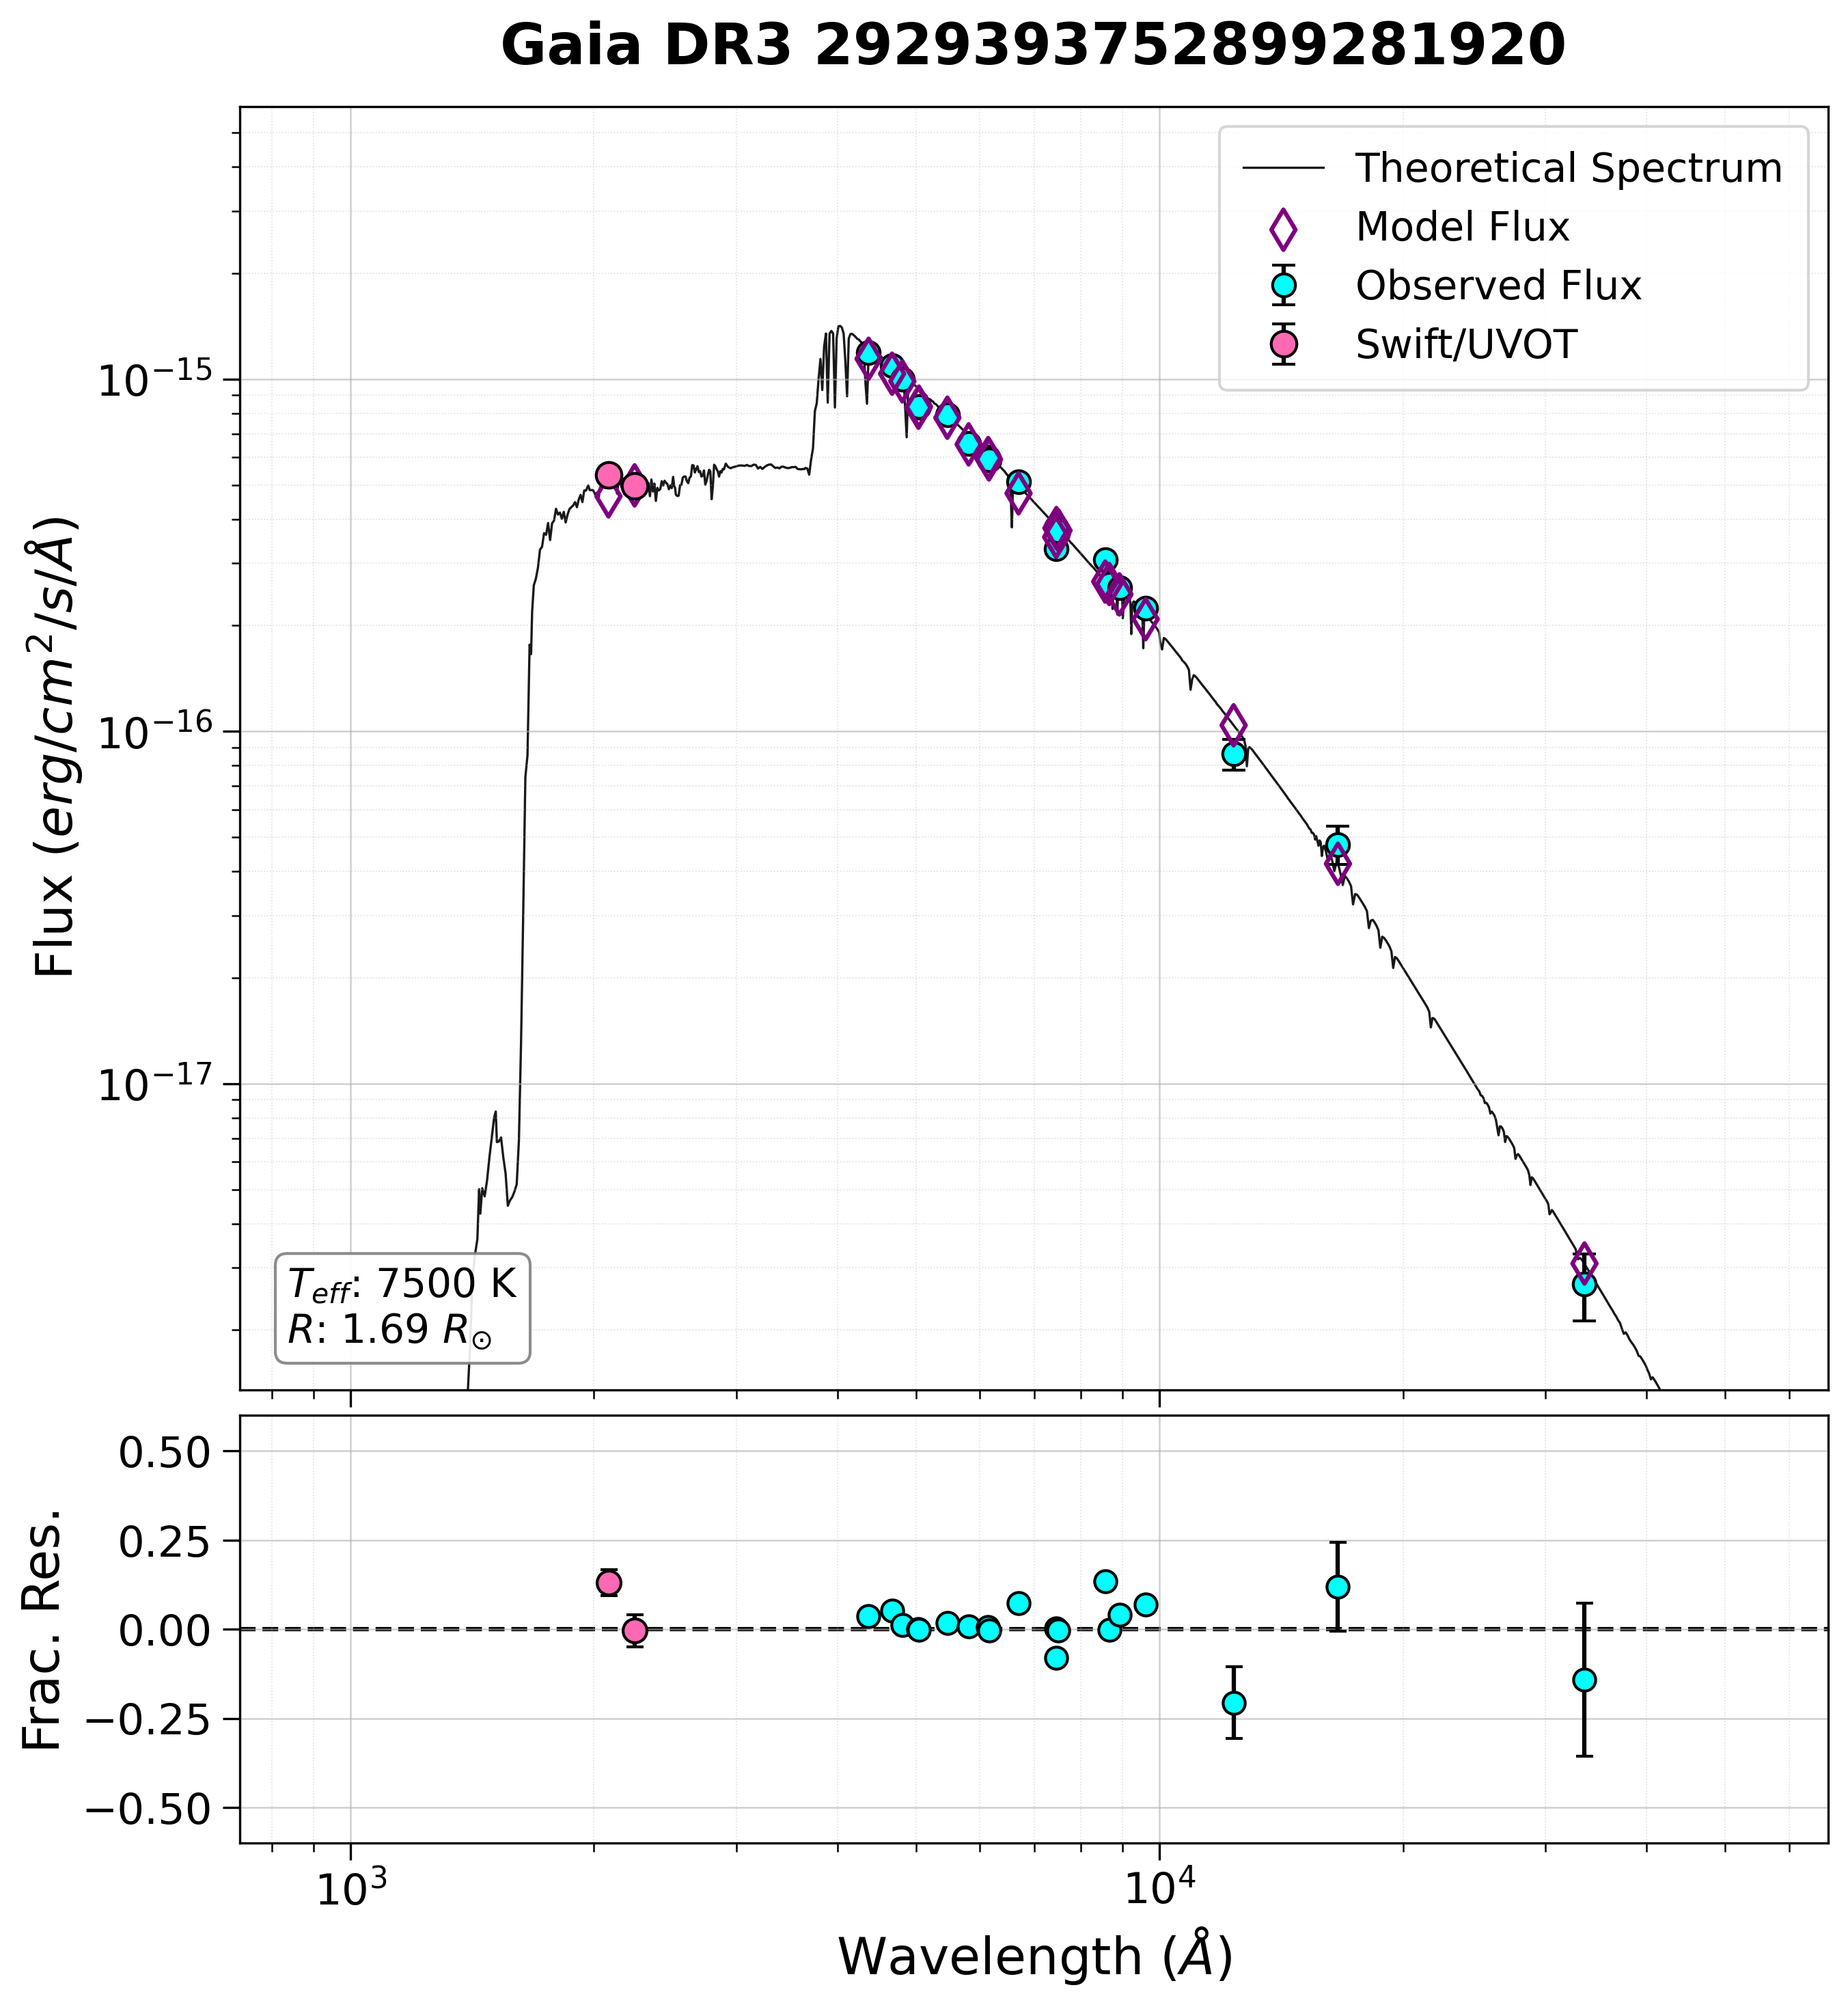}
%    \includegraphics[width=0.3\linewidth]{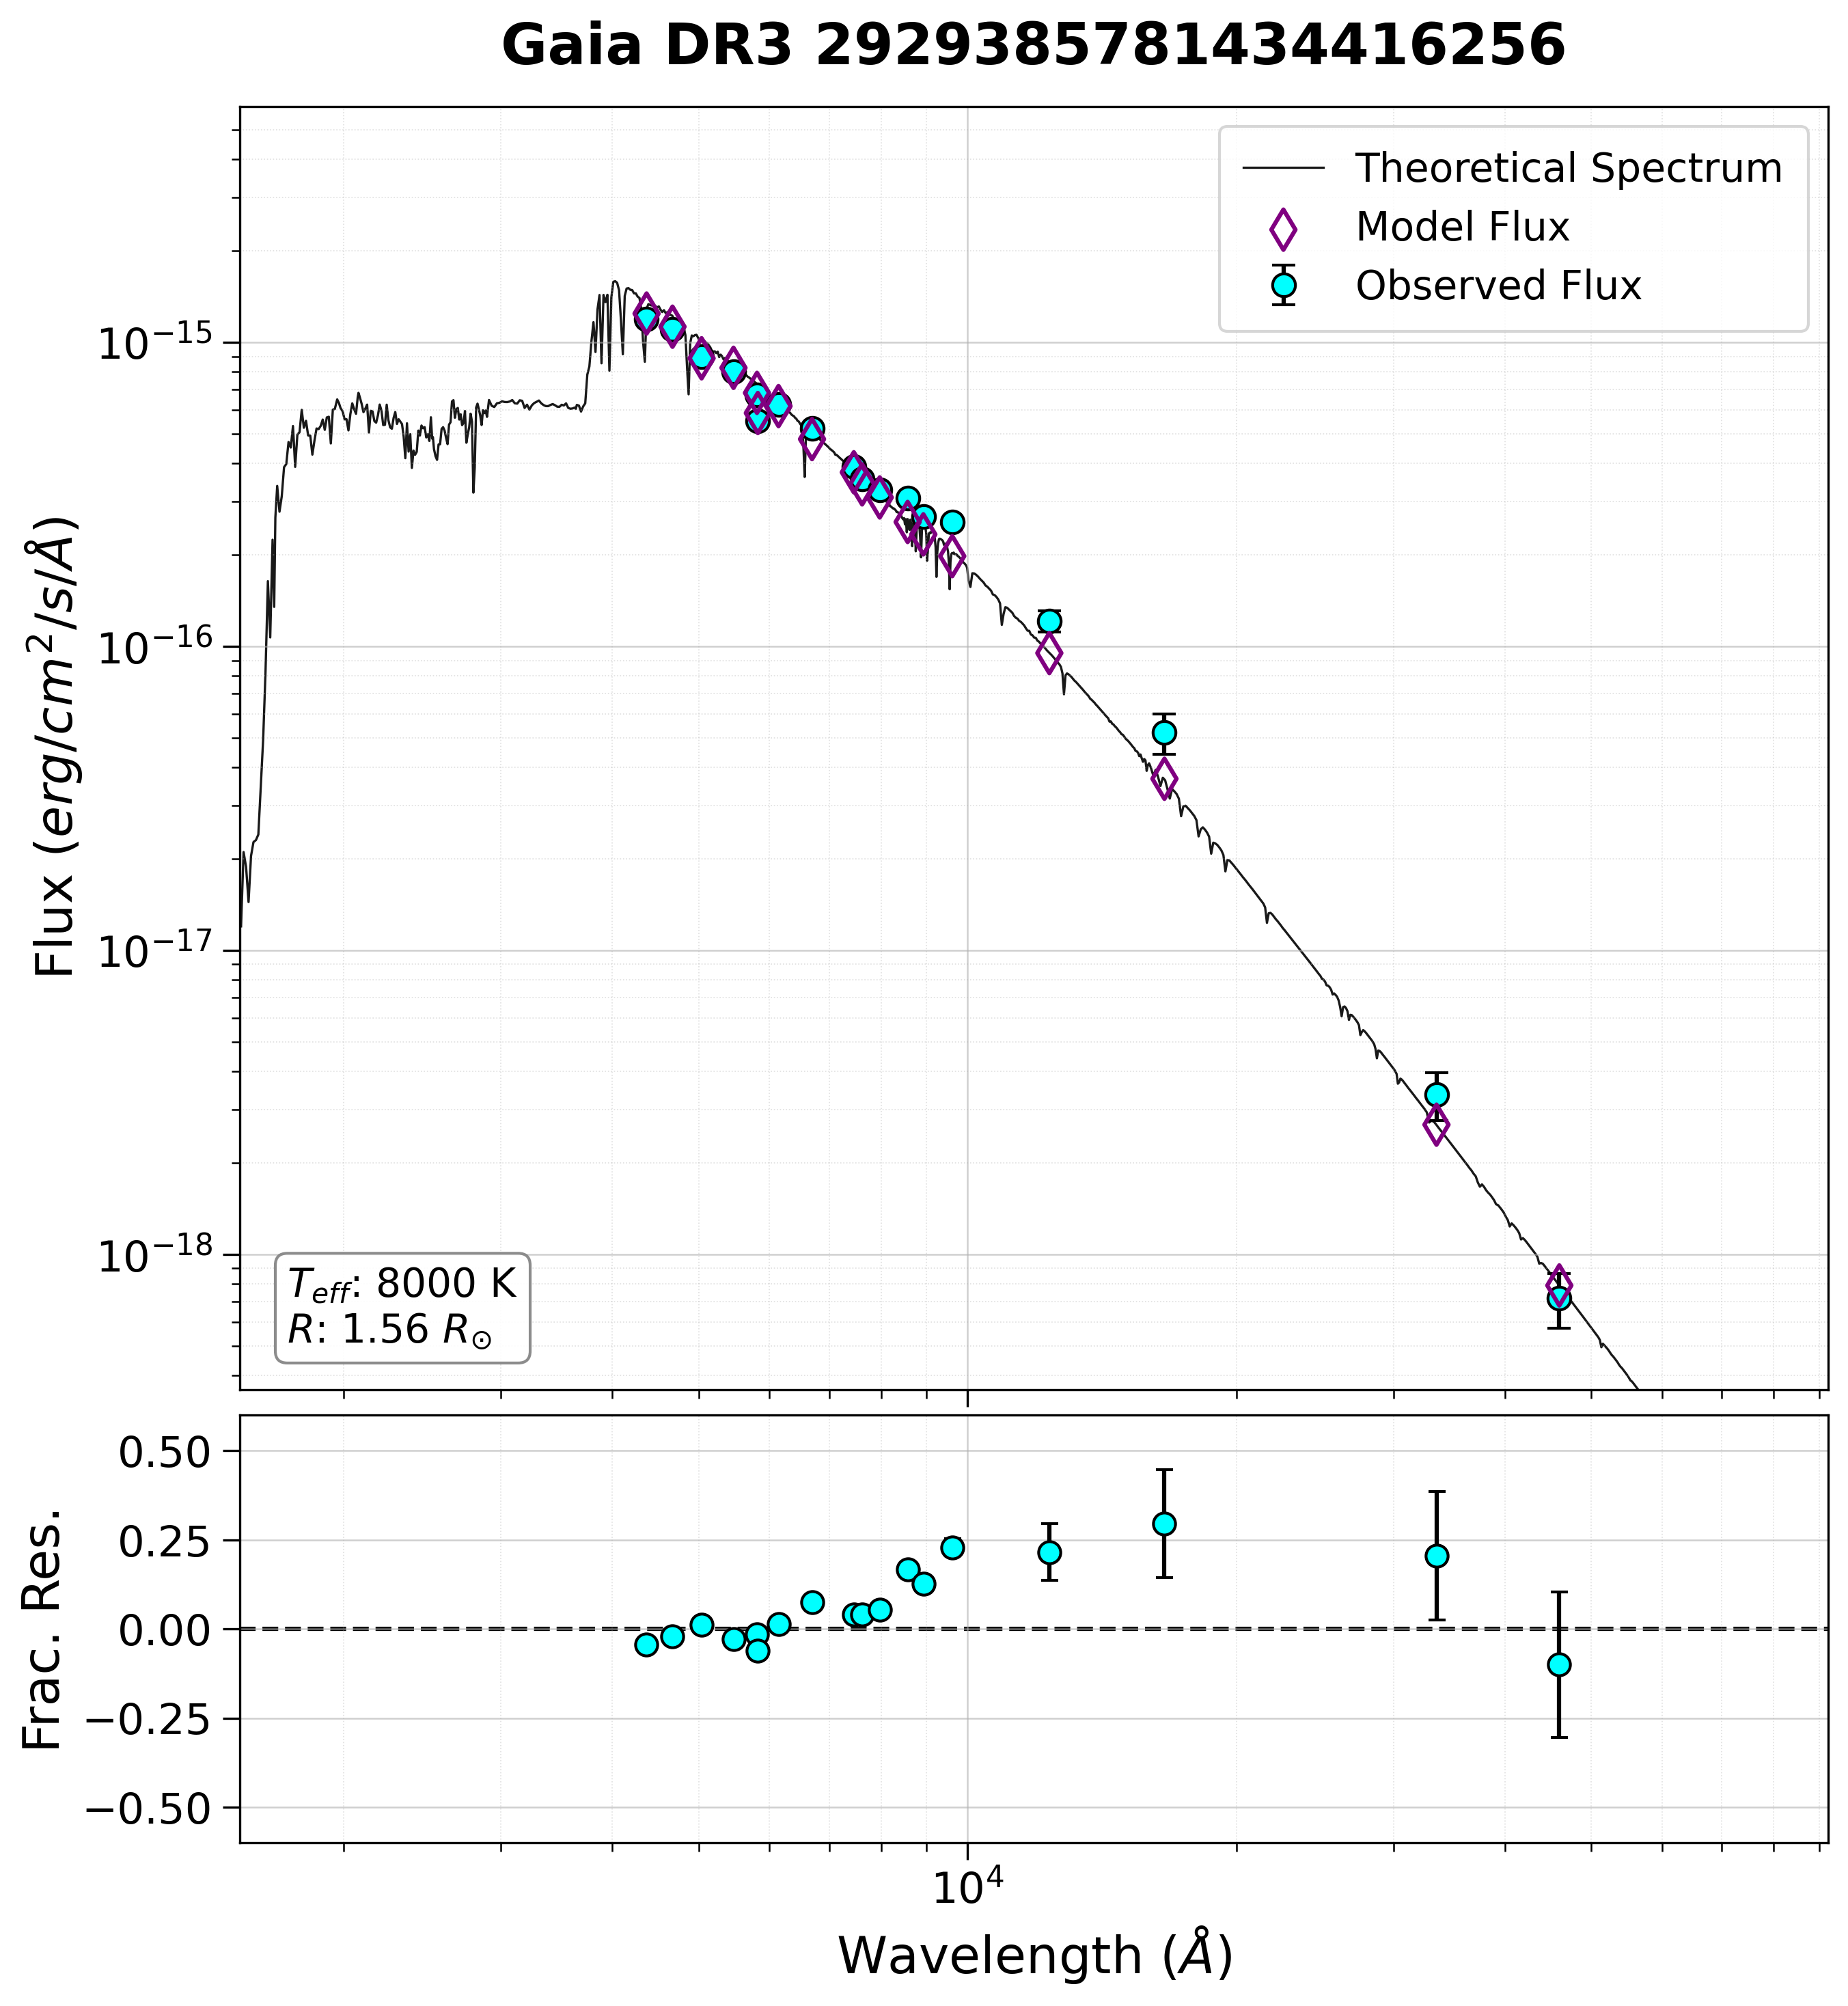}
%    \includegraphics[width=0.3\linewidth]{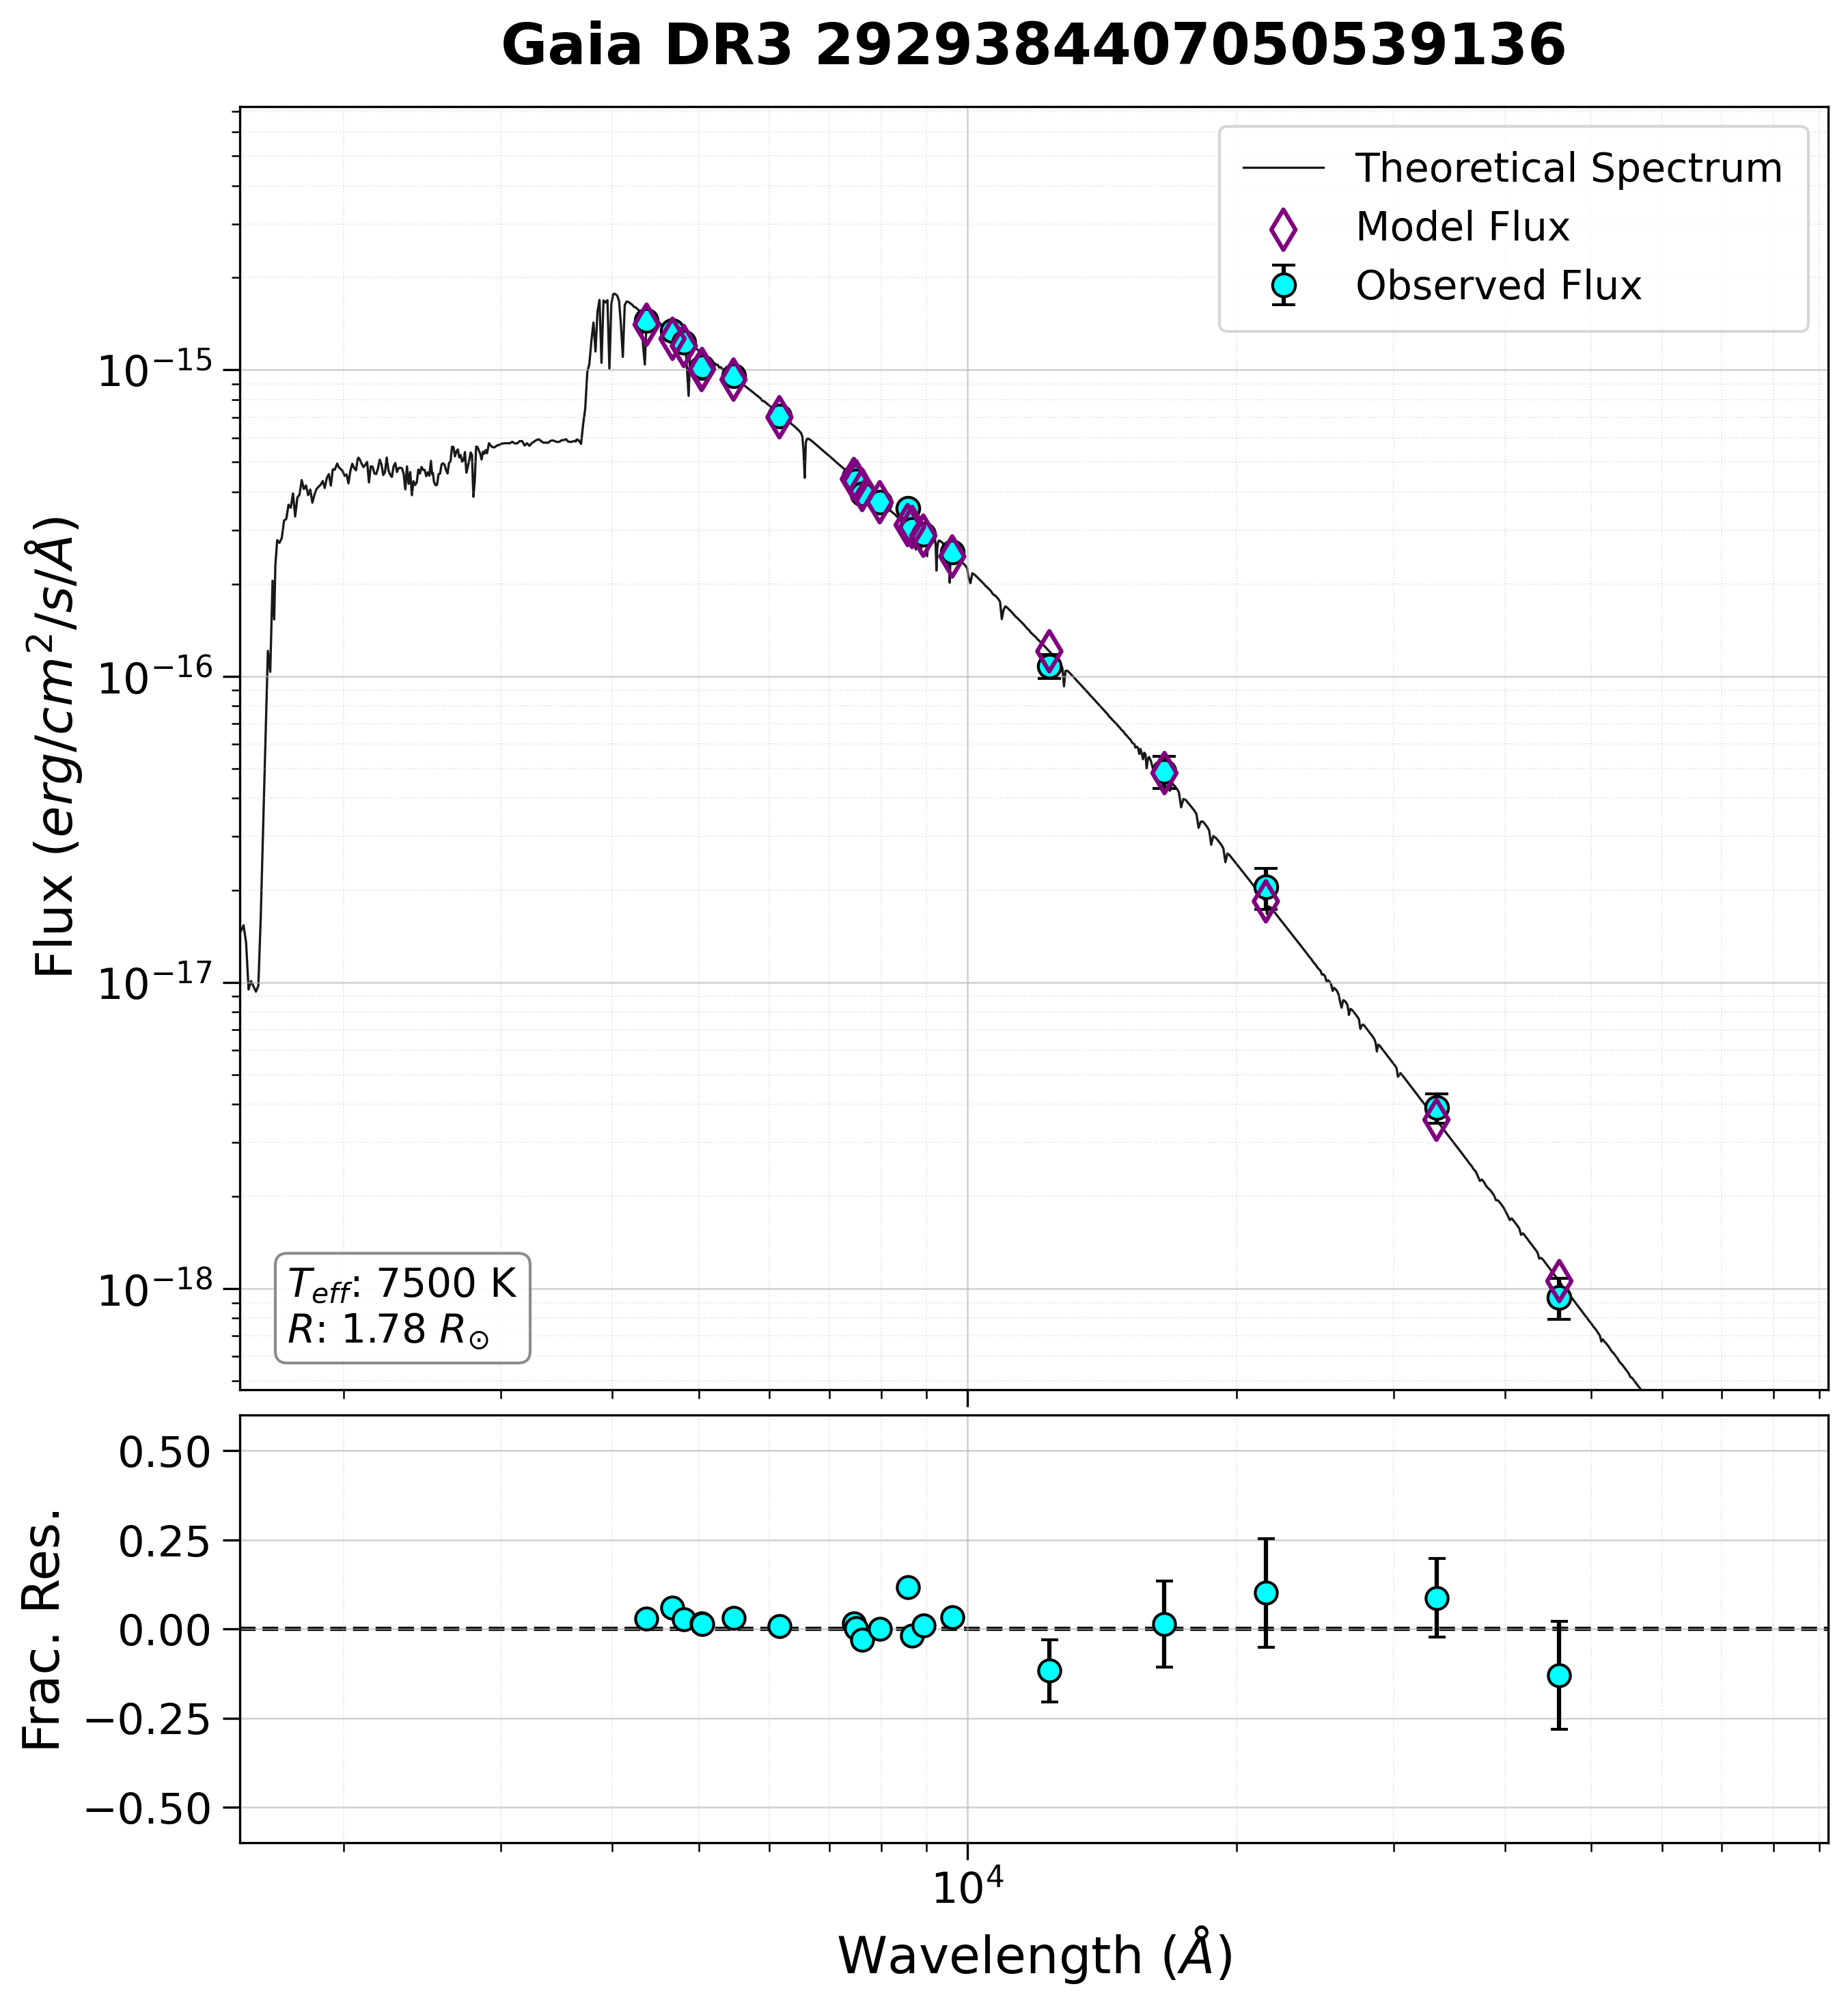}
%    \caption{Spectral energy distributions of blue straggler stars in Tombaugh 2 that are well fitted by single-component stellar models.}
%    \label{fig:placeholder}
%\end{figure*}

%\begin{figure*}
%    \centering
%    \includegraphics[width=0.3\linewidth]{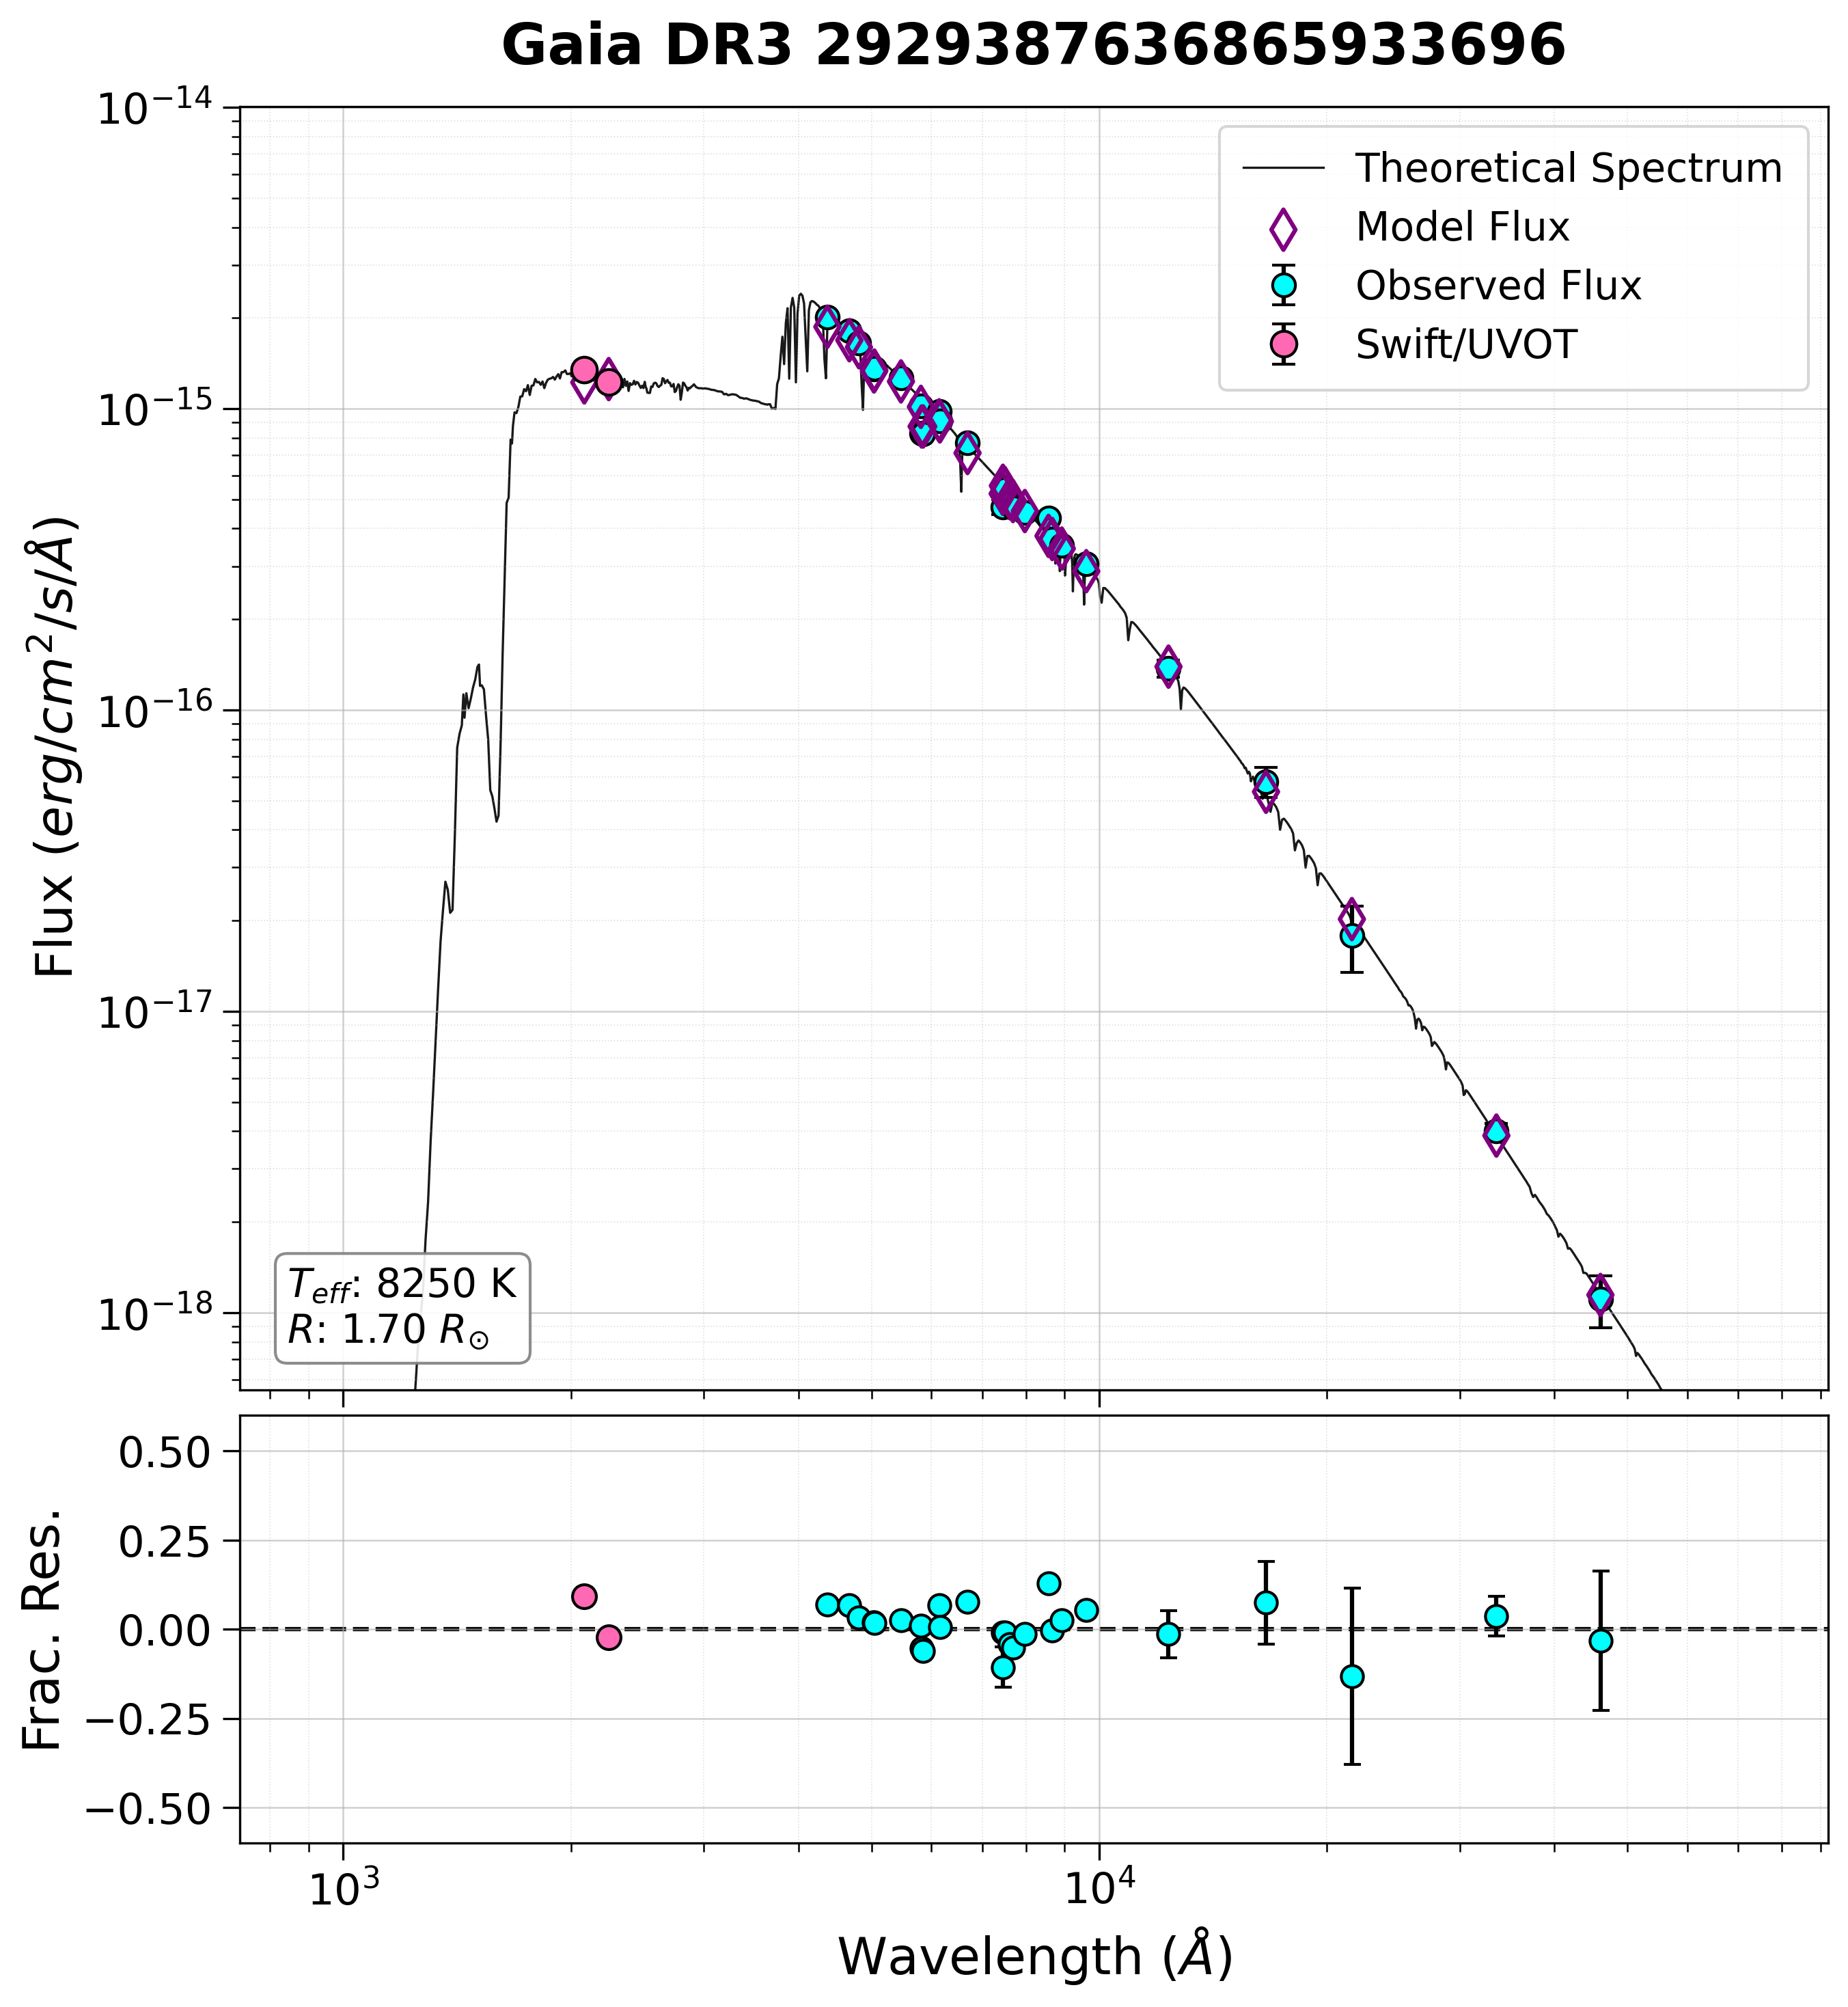}
%    \includegraphics[width=0.3\linewidth]{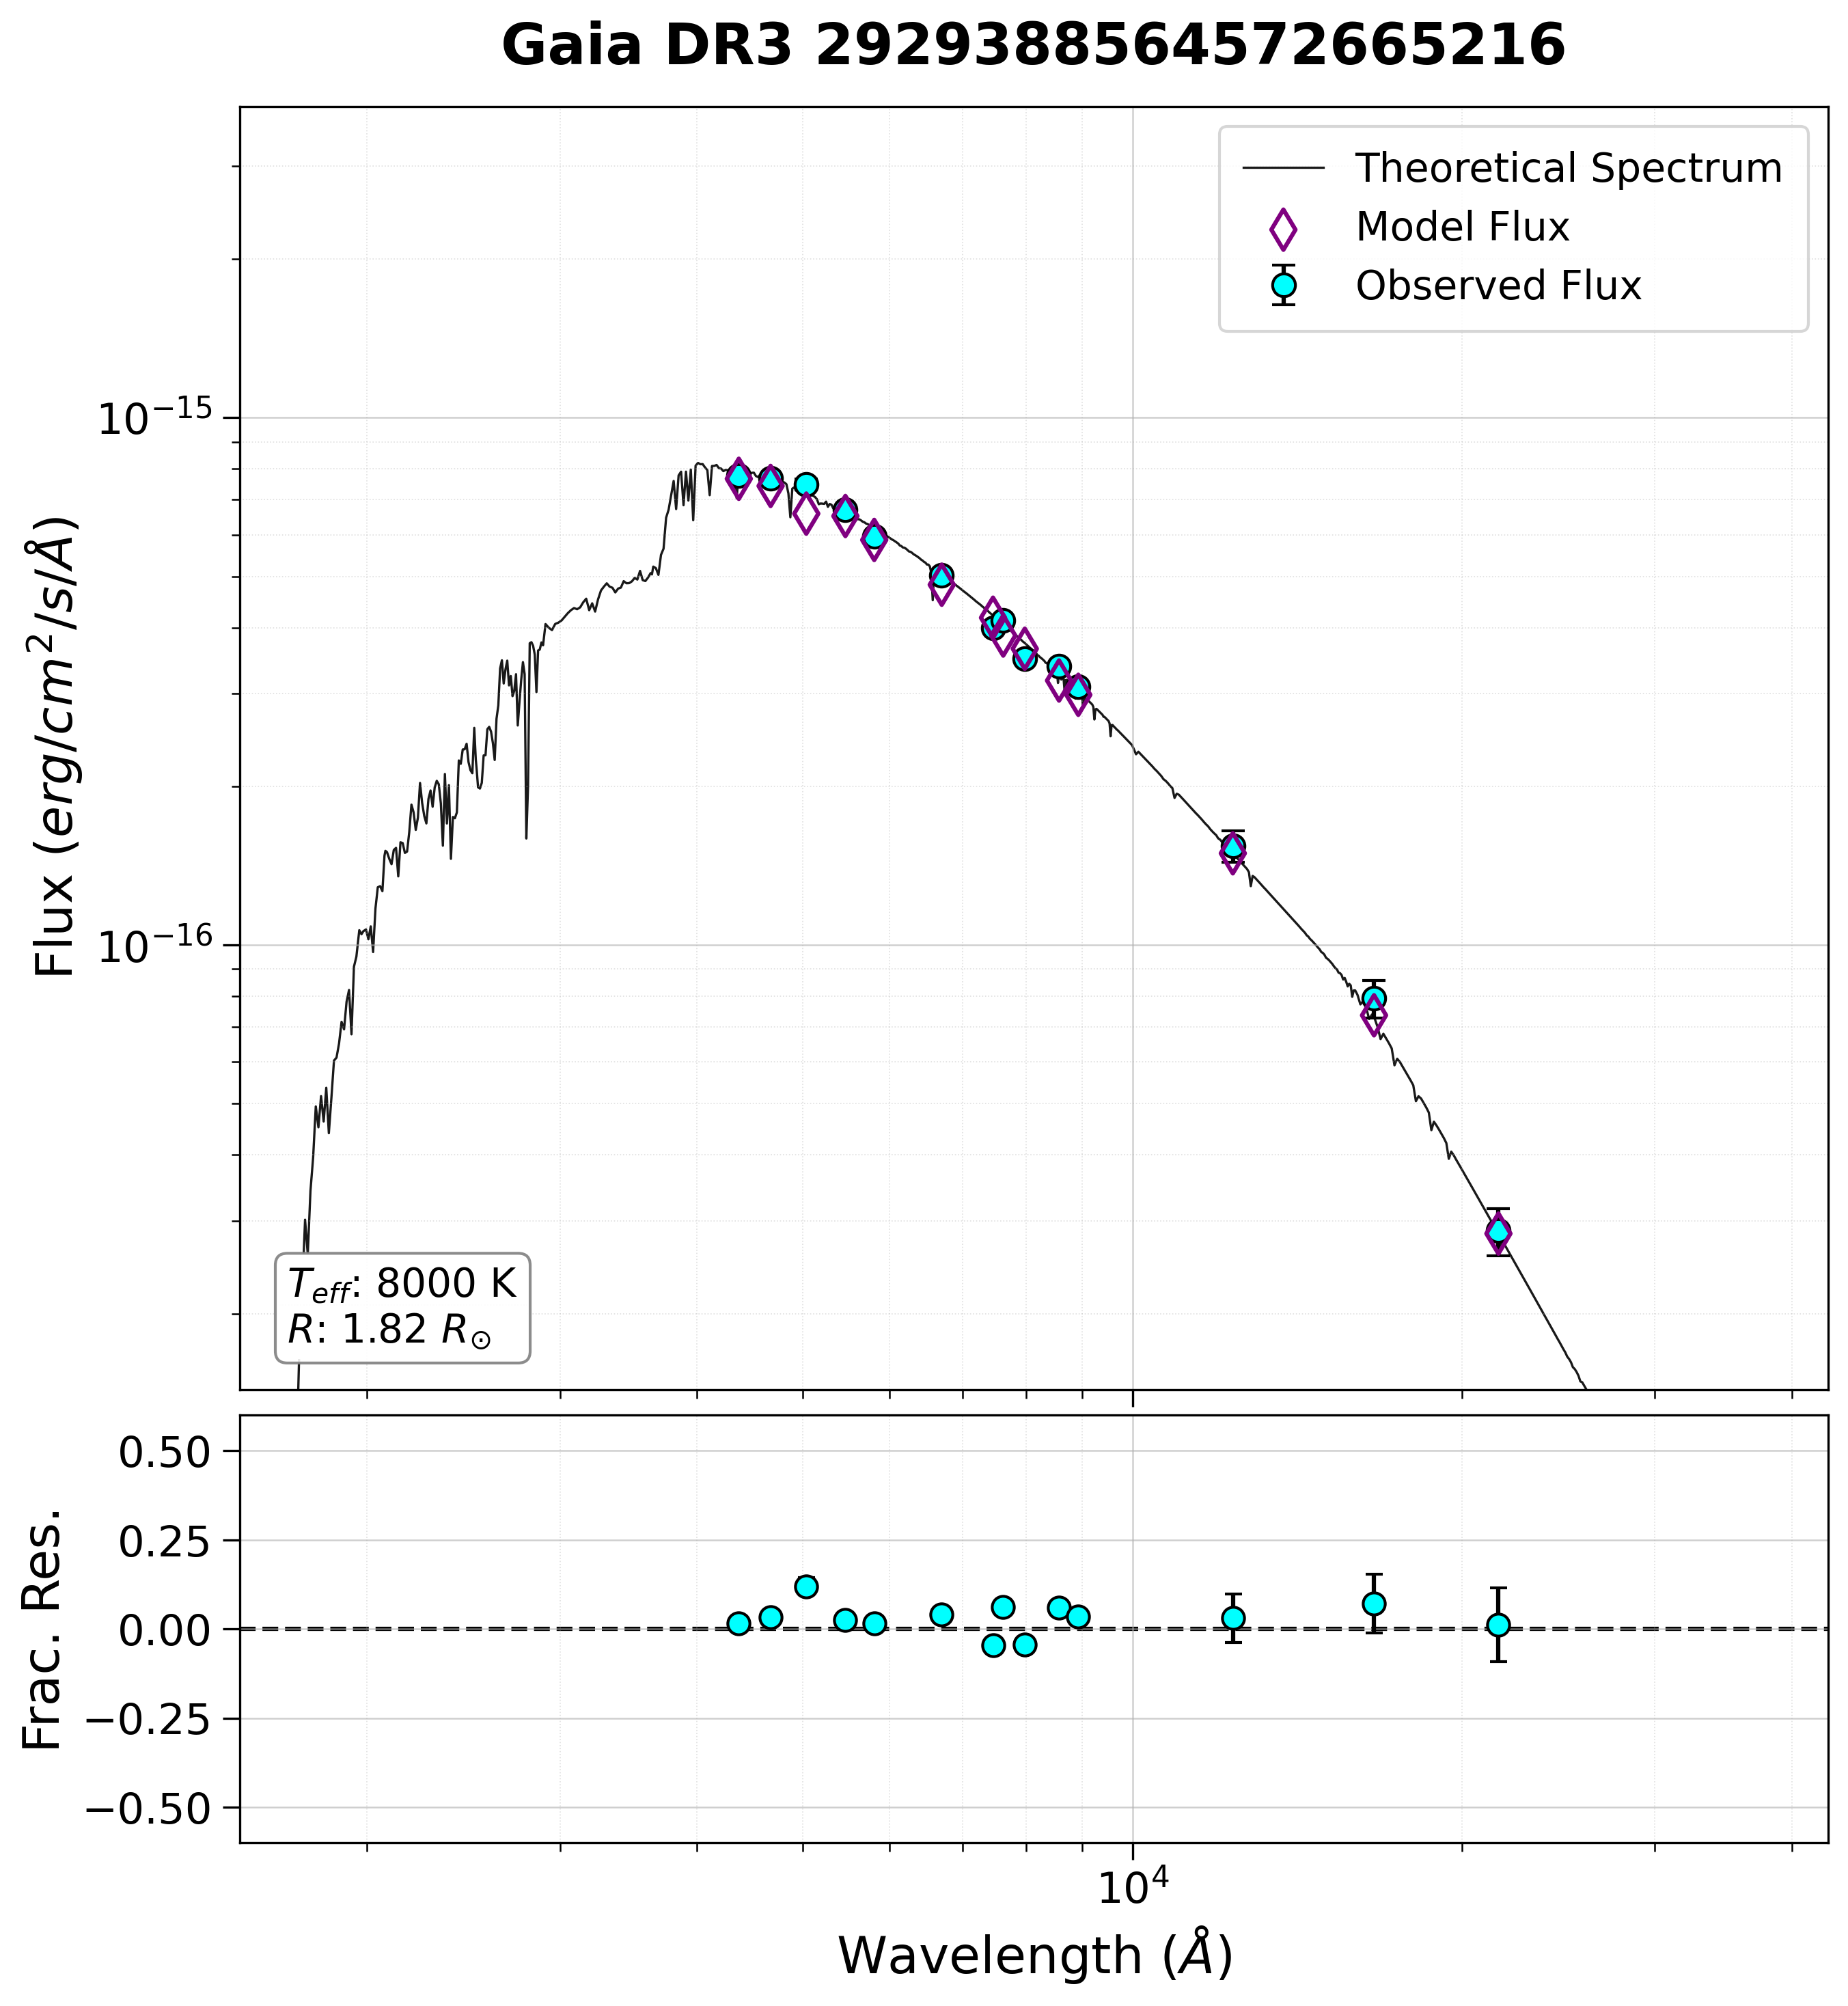}
%    \includegraphics[width=0.3\linewidth]{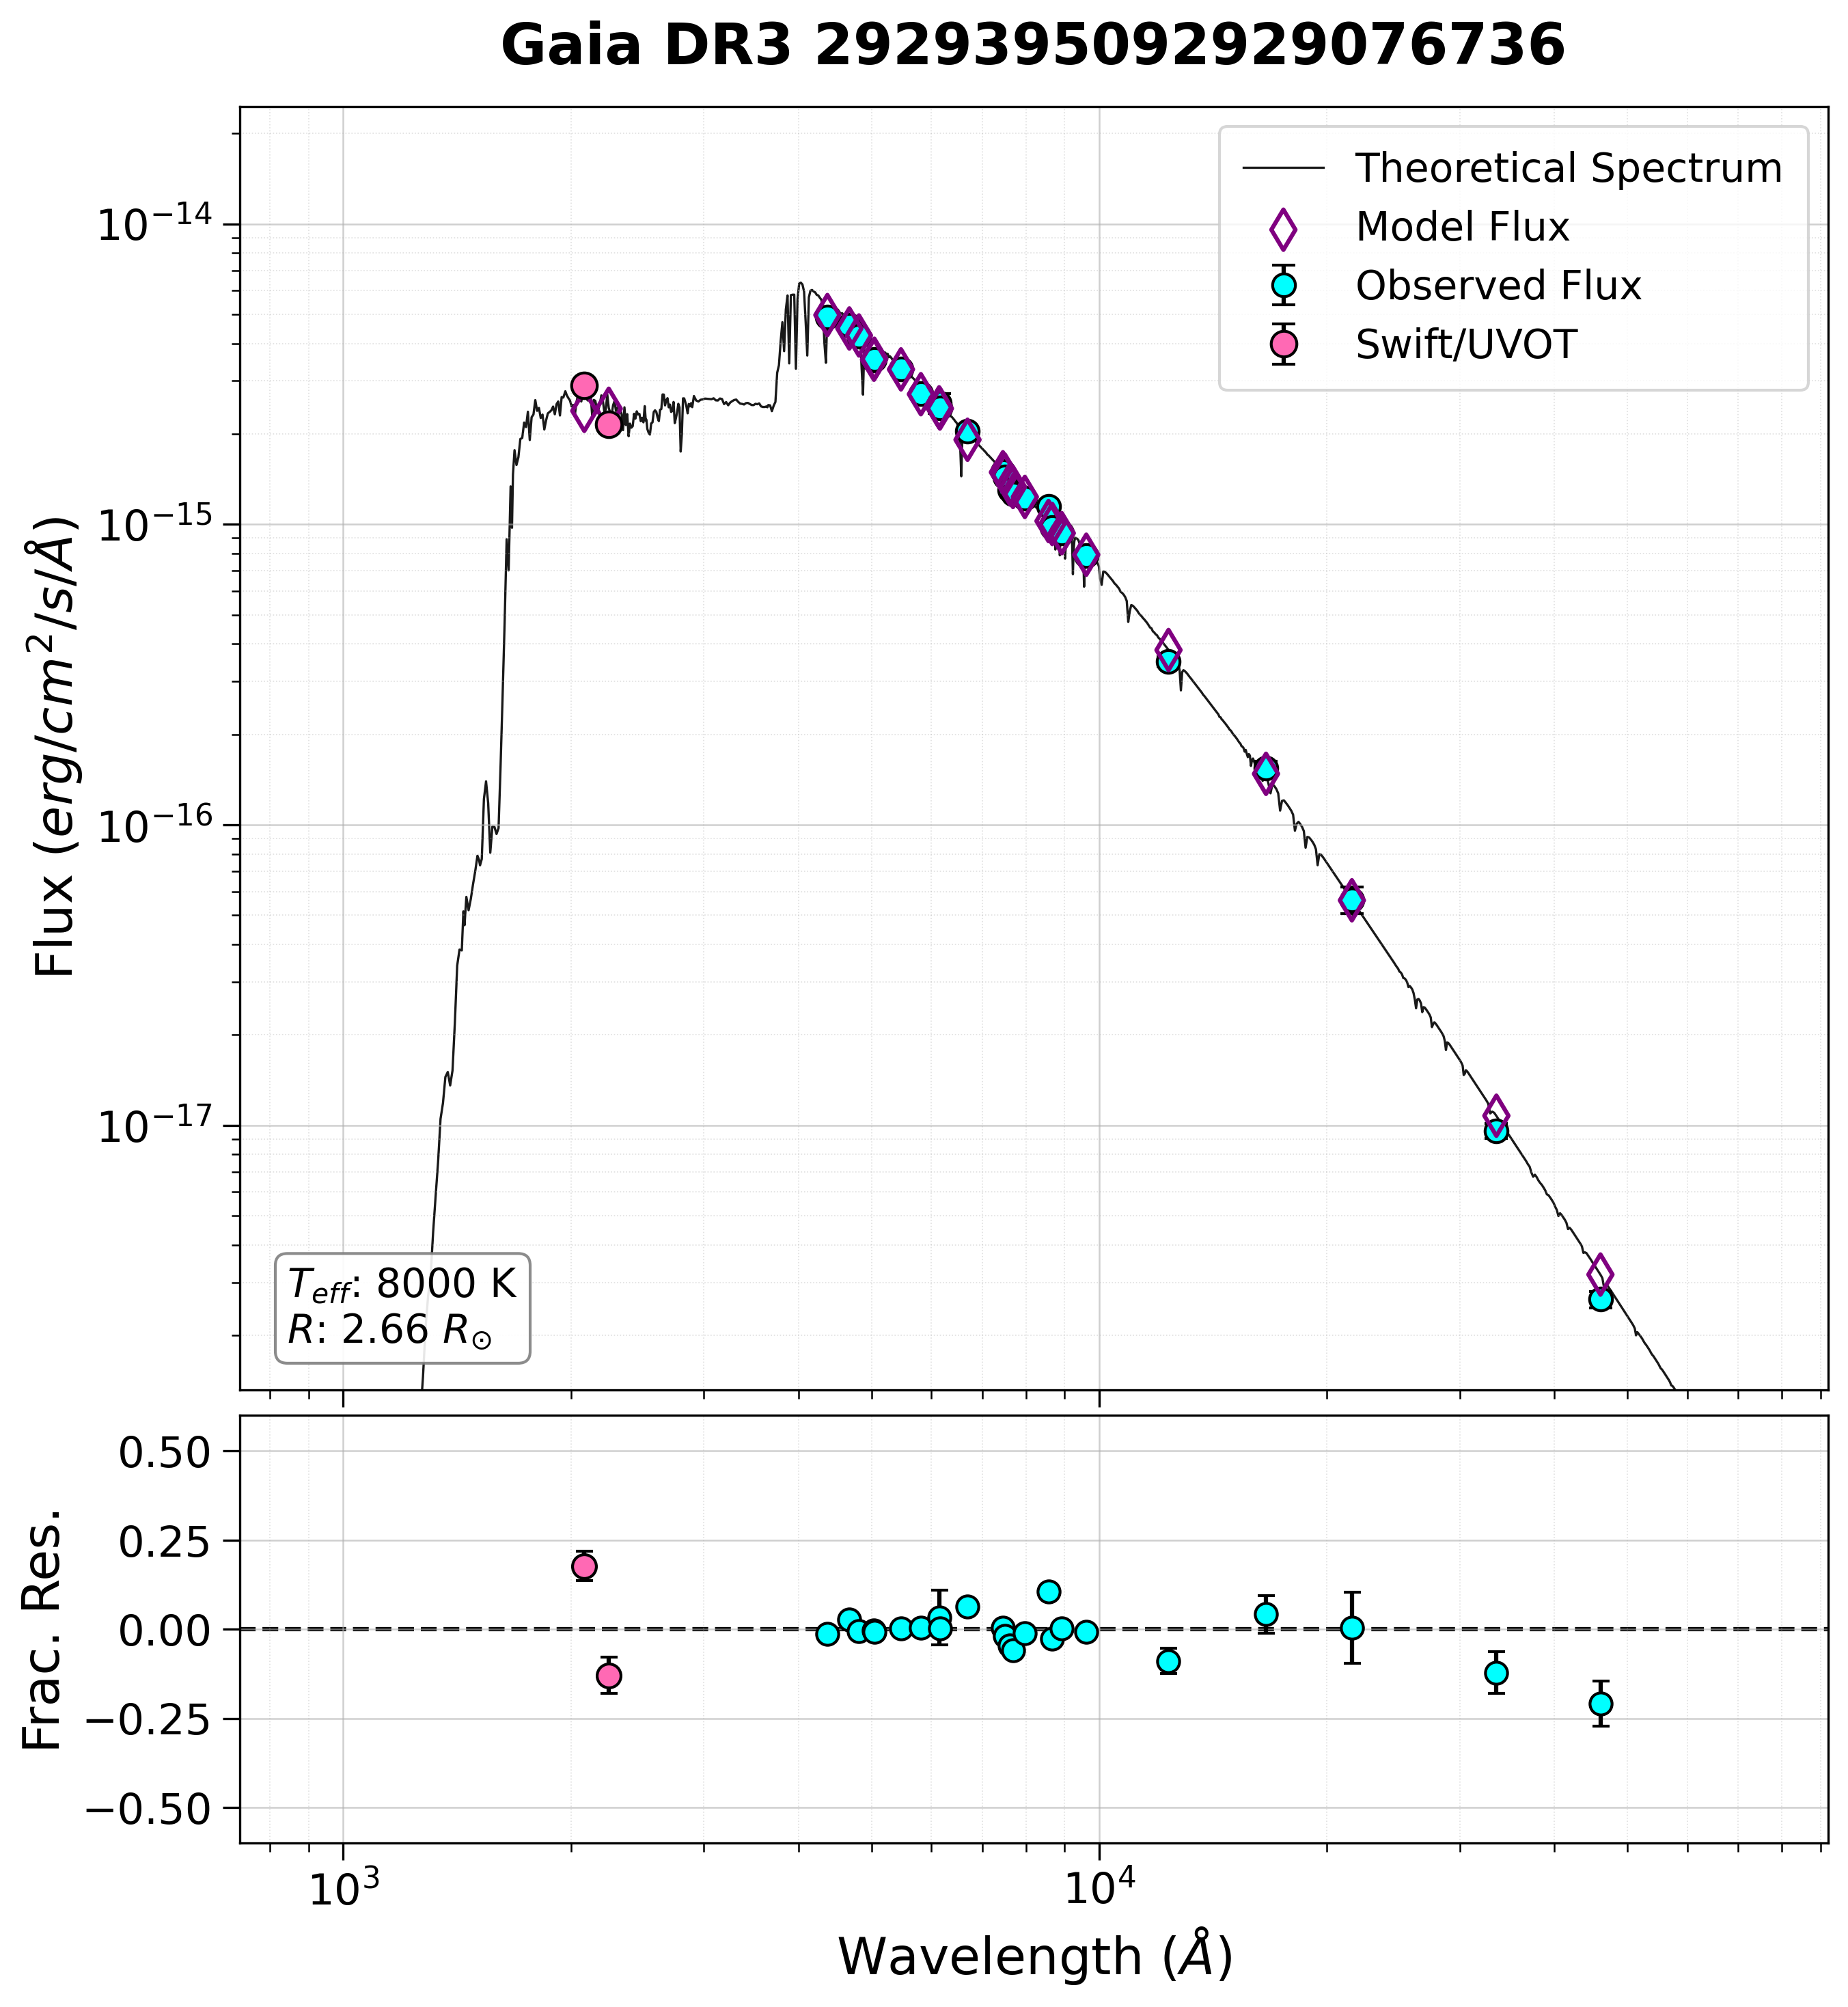}\\
%    \includegraphics[width=0.3\linewidth]{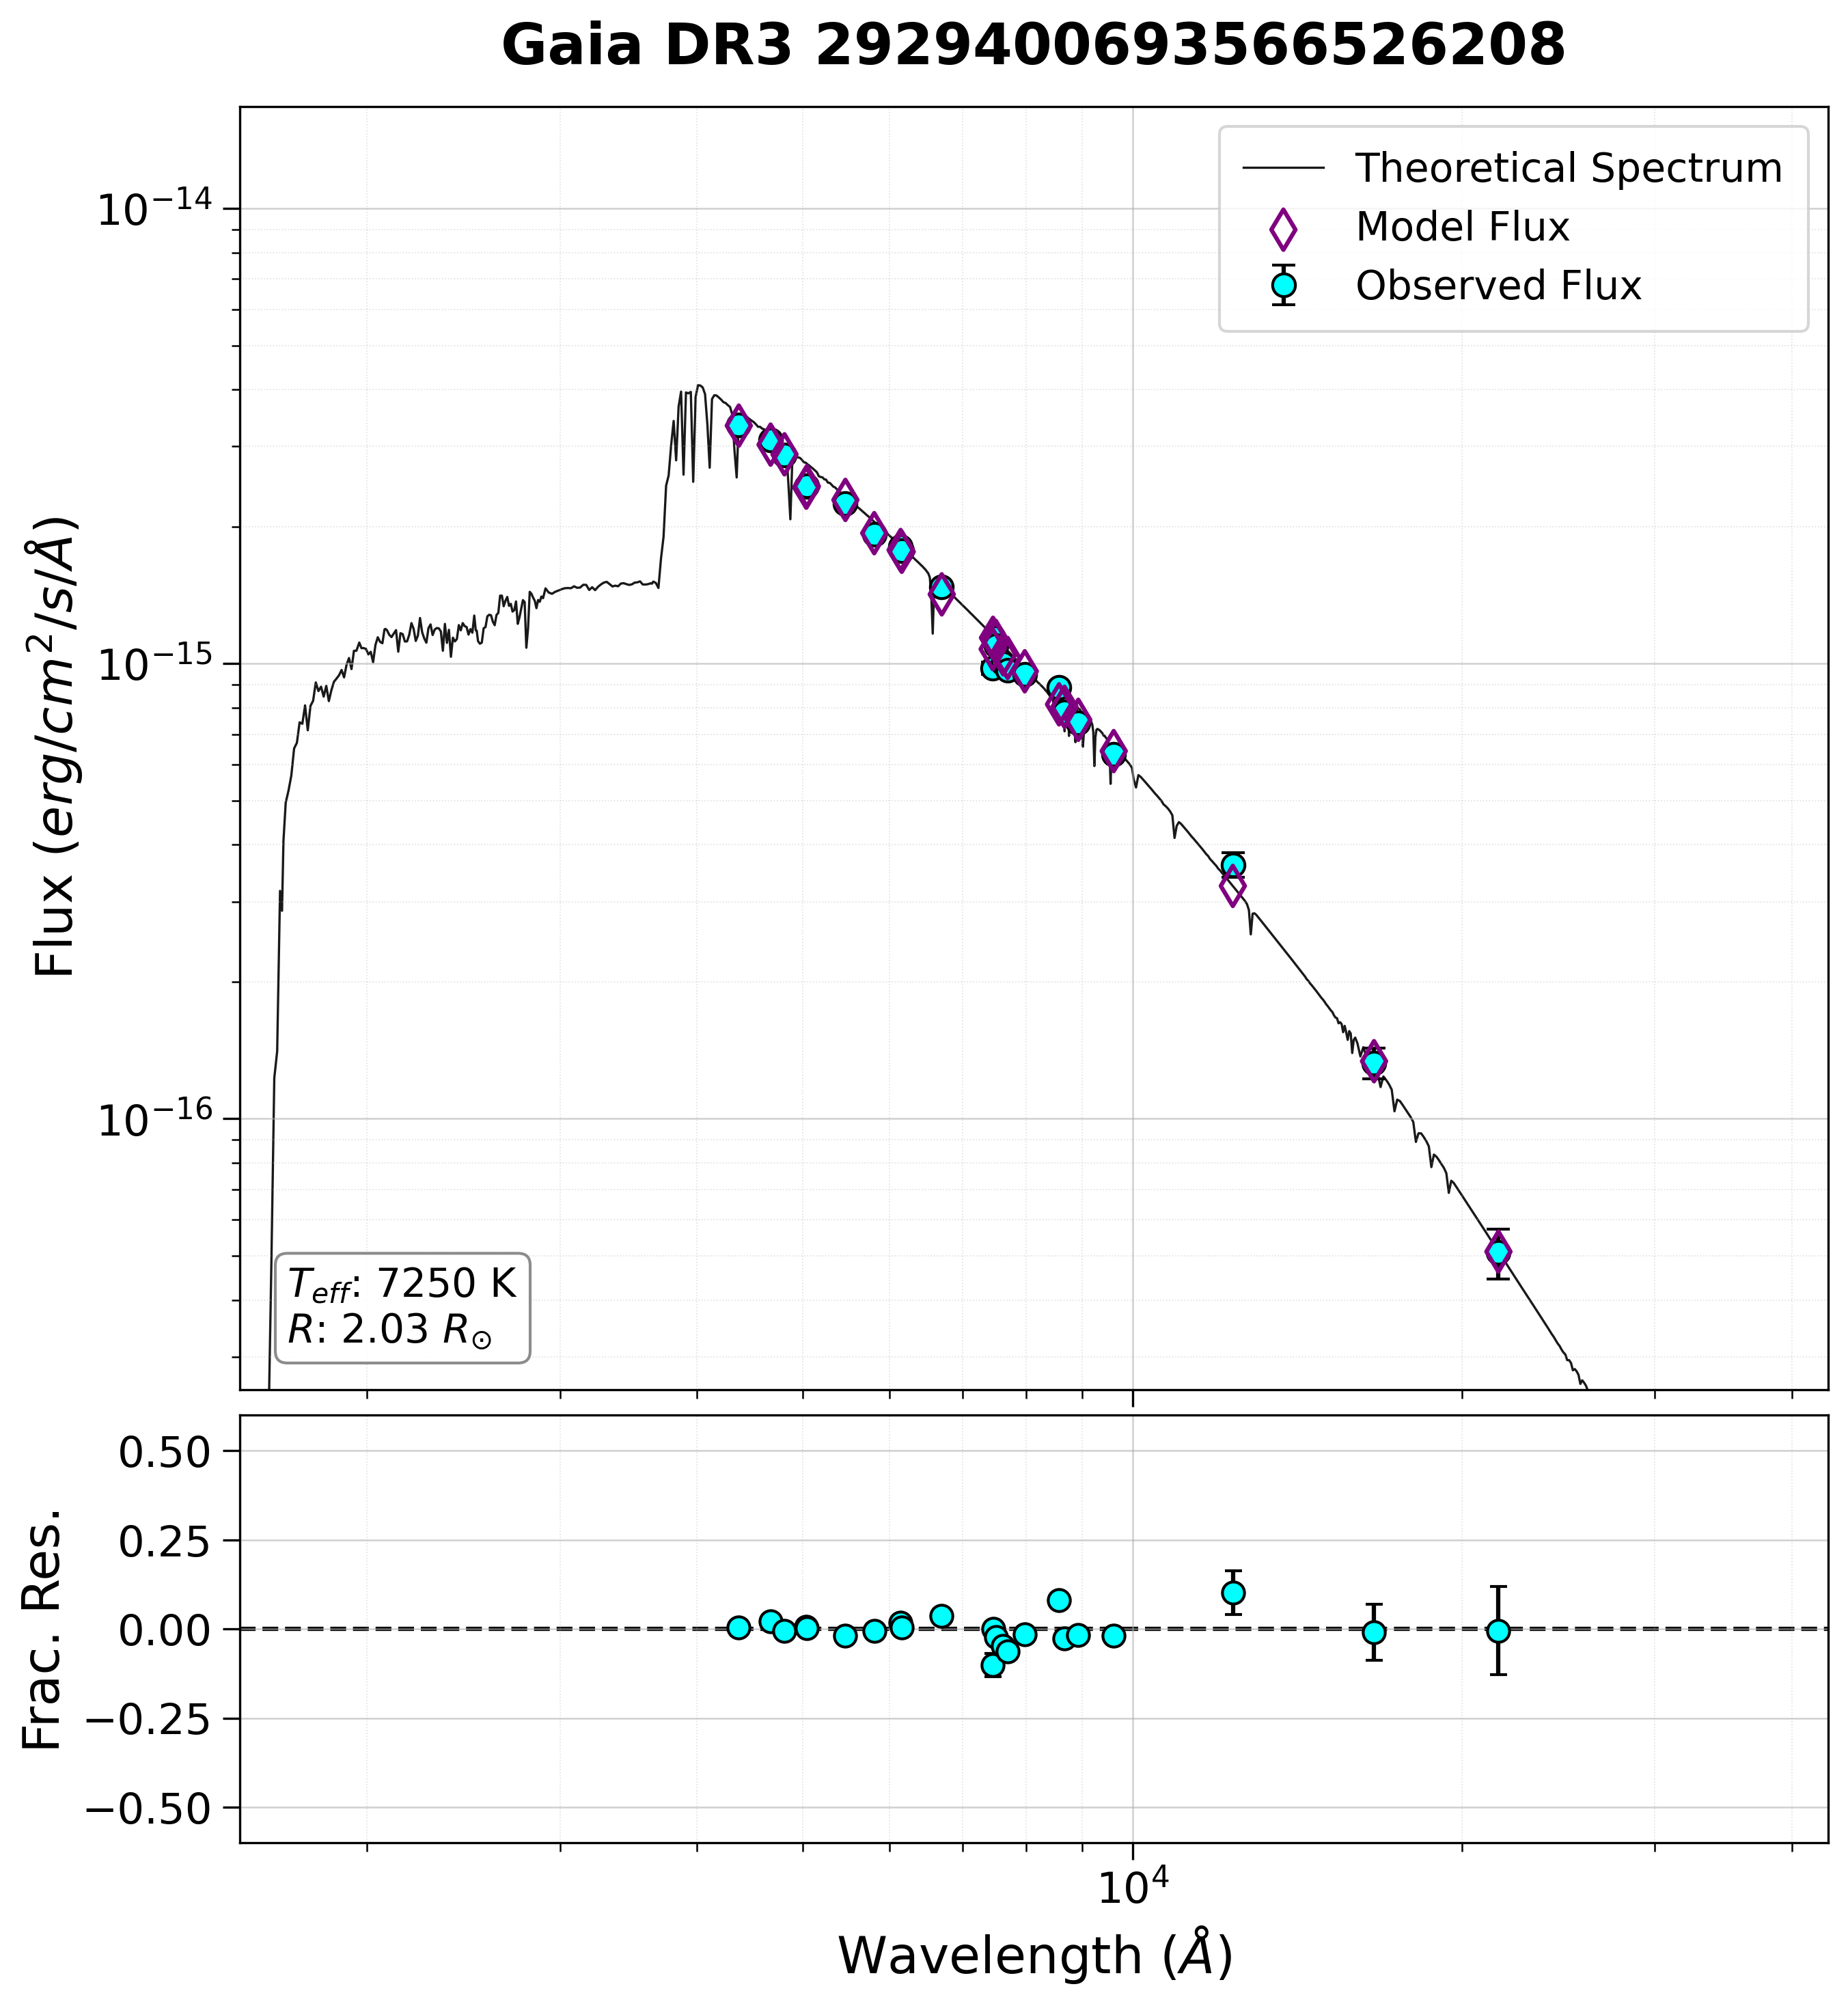}
%    \includegraphics[width=0.3\linewidth]{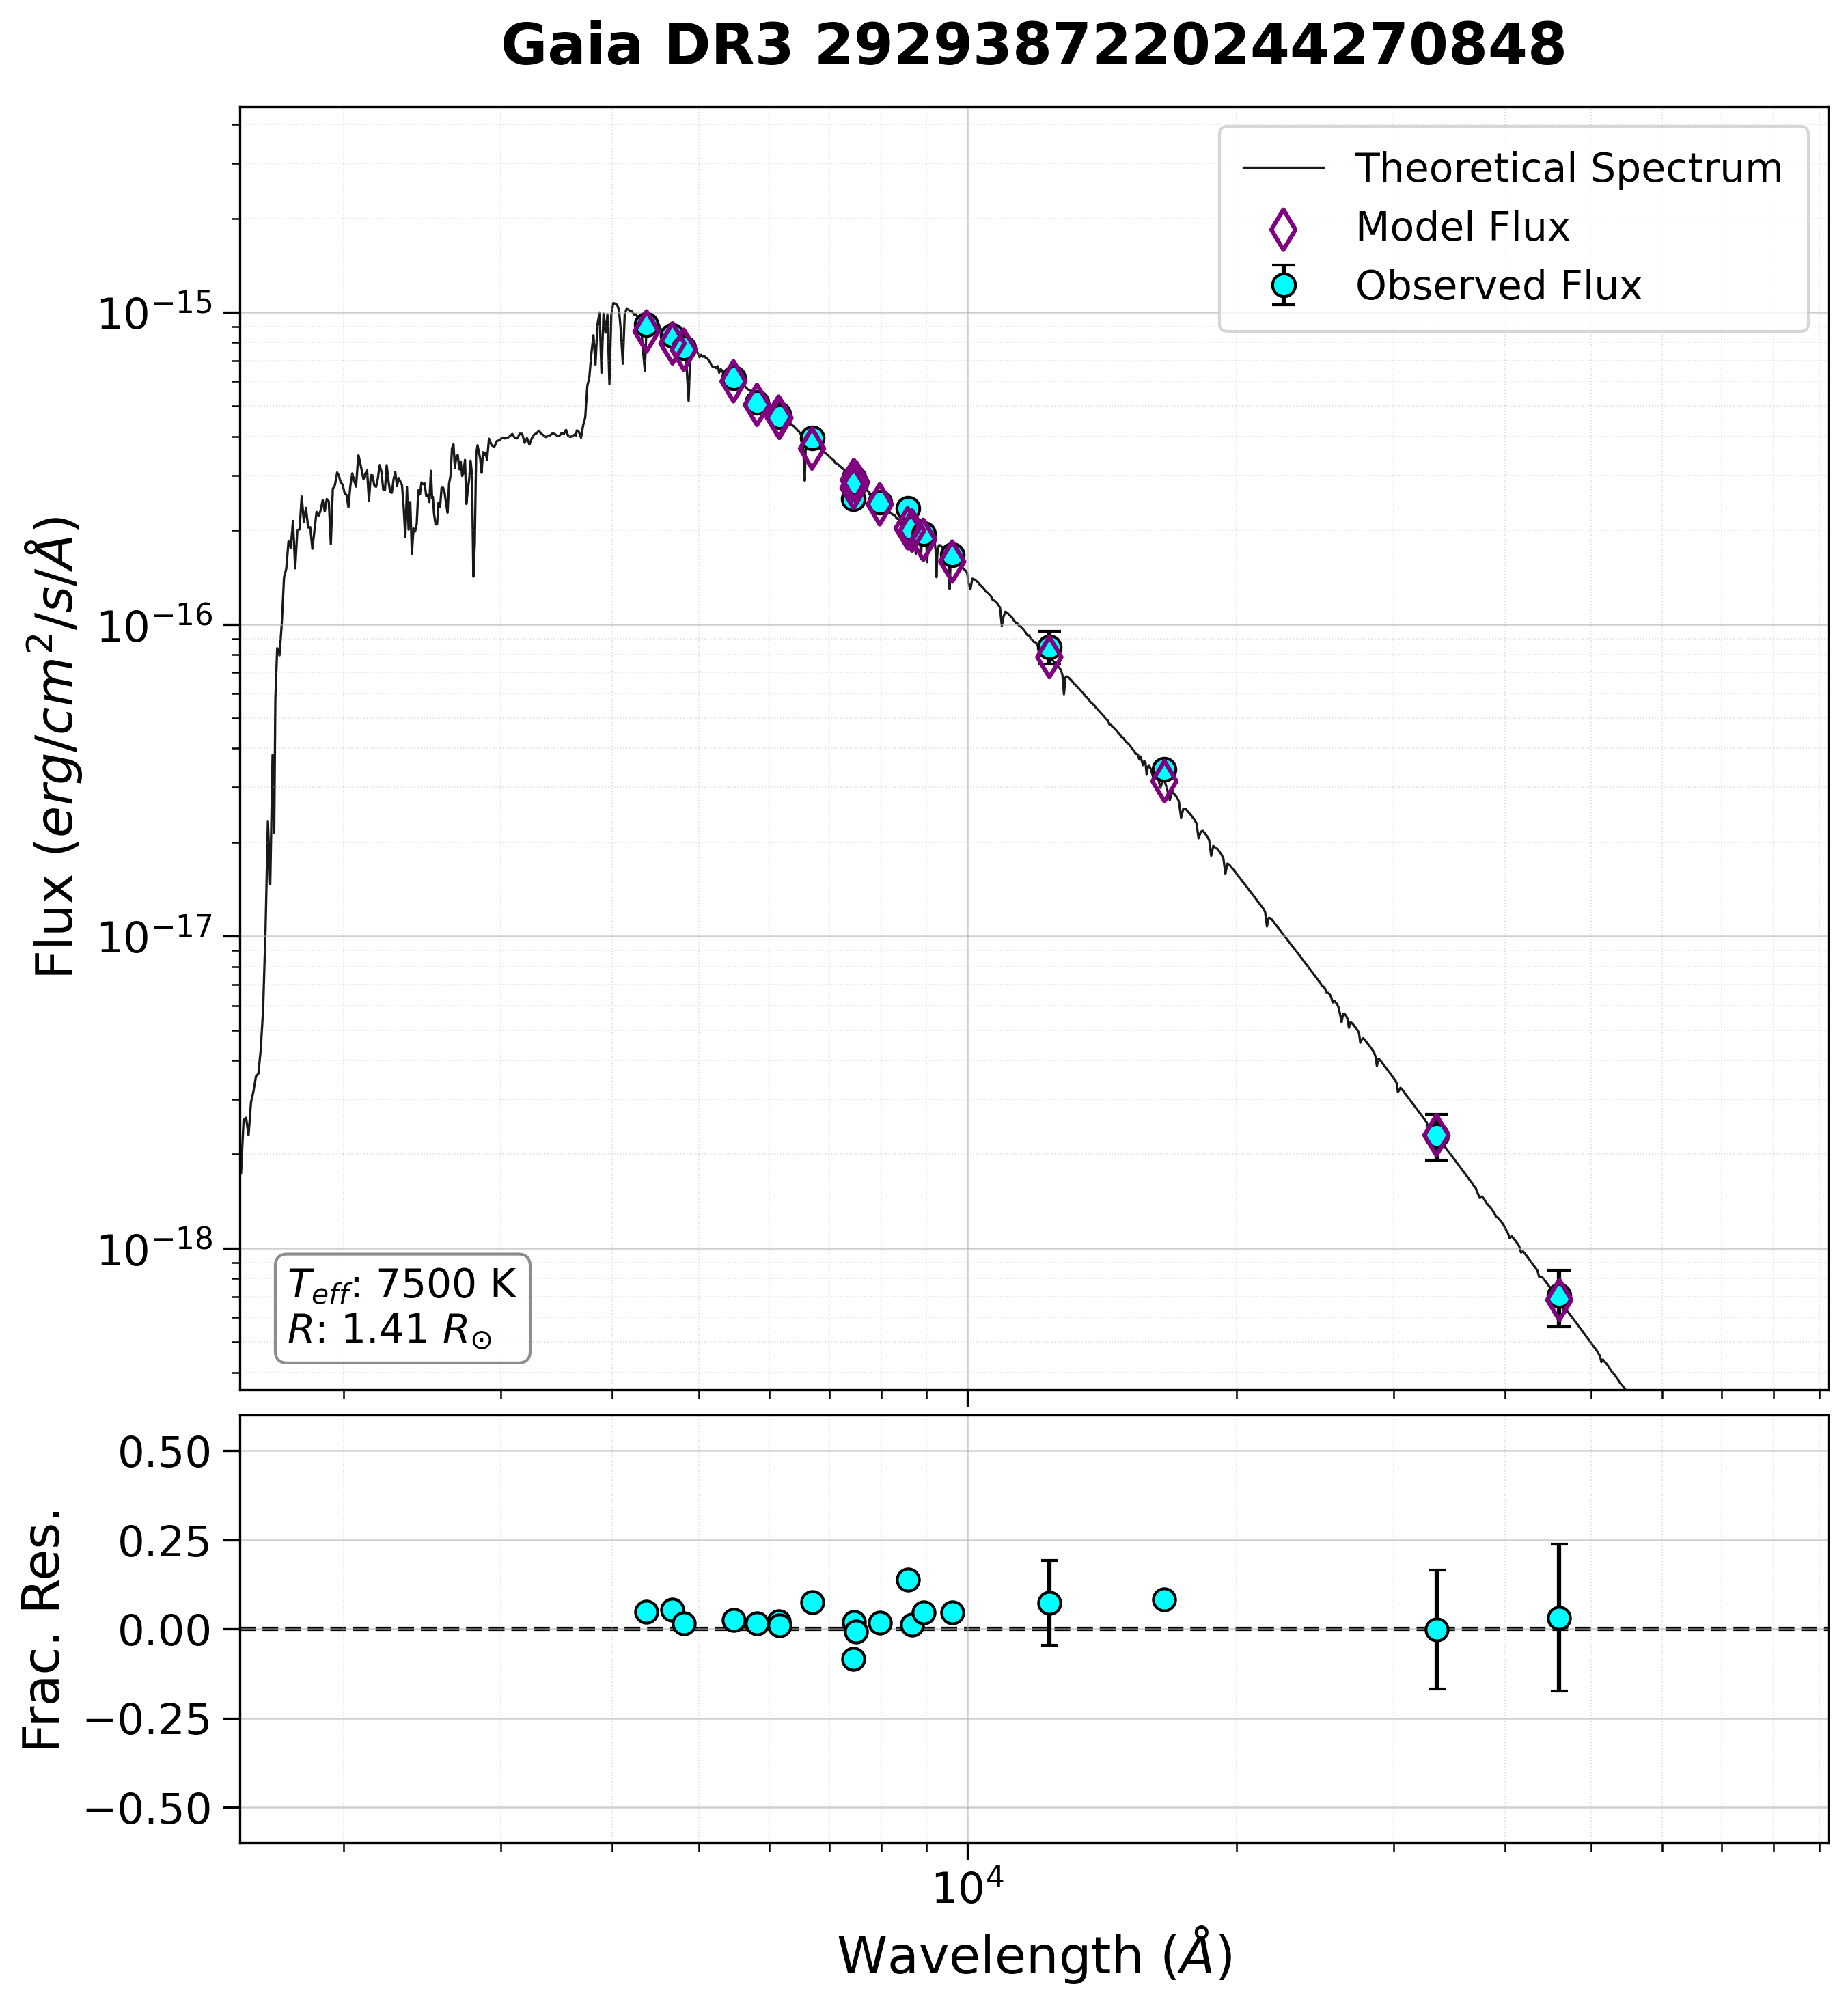}
%    \includegraphics[width=0.3\linewidth]{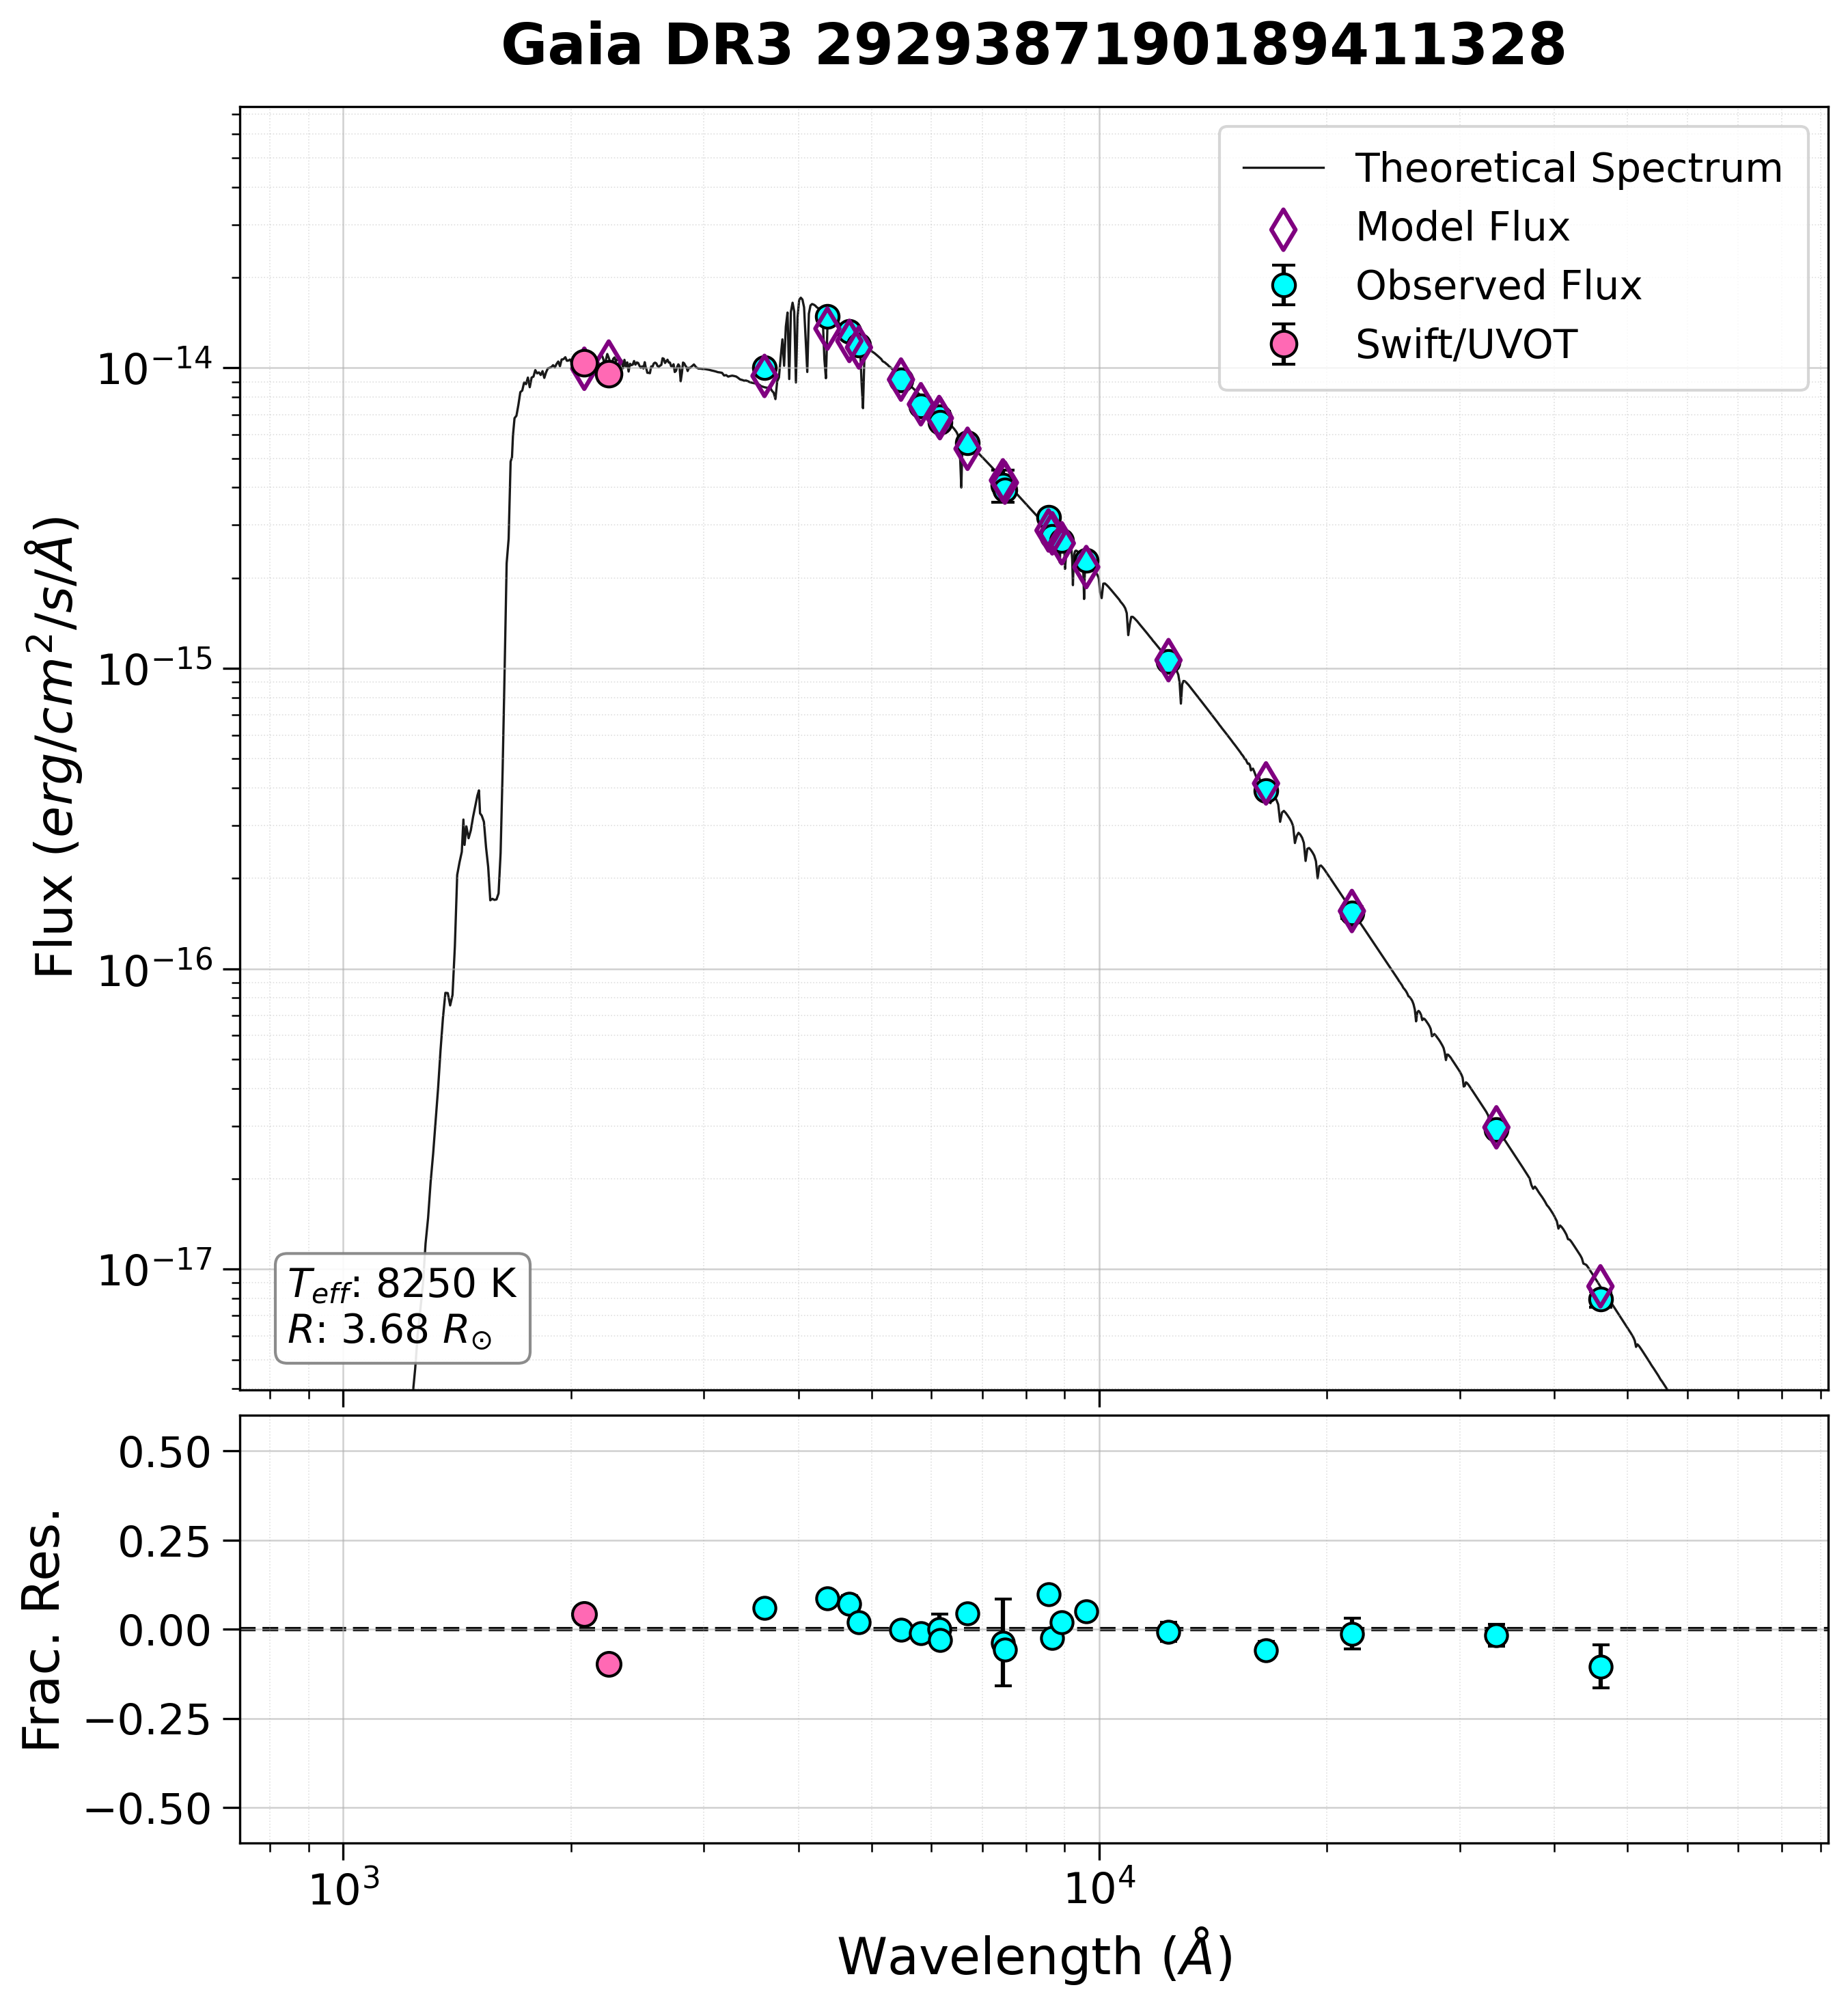}
%    \caption{(Continued.)}
%    \label{fig:placeholder}
%\end{figure*}
